# Supplementary material for: Cohesion and Repulsion in Bayesian Distance Clustering
Source: arXiv:2107.05414 ancillary file (2023-04-03)
Supplement: Supplementary file 1 [file Supplementary_Materials.pdf]

# Supplementary Material
# Cohesion and Repulsion in Bayesian Distance Clustering


Abhinav Natarajan
University of Oxford

Maria De Iorio
National University of Singapore

Andreas Heinecke
Yale-NUS College

Emanuel Mayer
Yale-NUS College

Simon Glenn
University of Oxford


## 1 Proof of Proposition 1

The probability generating function for each $n_j$ conditional on $r, p$ is

$$PGF(t) = t\left(\frac{1-p}{1-pt}\right)^r$$

and hence the conditional PGF for $n_1 + \ldots + n_K$ is

$$\begin{aligned} PGF(t) &= t^K \left(\frac{1-p}{1-pt}\right)^{rK} \\ &= \sum_{j=0}^{\infty} (1-p)^{rK} p^j \frac{\Gamma(rK+j)}{\Gamma(rK)\Gamma(j+1)} t^{j+K} \end{aligned}$$


Abhinav Natarajan is a doctoral student at the Mathematical Institute, University of Oxford, United Kingdom OX1 2JD (E-mail: *natarajan@maths.ox.ac.uk*). Maria De Iorio is Professor at Yong Loo Lin School of Medicine, National University of Singapore, Singapore 138527, Professor of Biostatistics at University College London and Principal Investigator at A*STAR, Singapore 138632 (E-mail: *mdi@nus.edu.sg*). Andreas Heinecke is Assistant Professor of Mathematics at Yale-NUS College, Singapore 138527 (E-mail: *andreas.heinecke@yale-nus.edu.sg*). Emanuel Mayer is Associate Professor of History at Yale-NUS College, Singapore 138527 (E-mail: *emanuel.mayer@yale-nus.edu.sg*). Simon Glenn is Research Fellow at the Ashmolean Museum, University of Oxford, United Kingdom OX1 2PH (E-mail: *simon.glenn@ashmus.ox.ac.uk*).

Therefore for $1 \leq K \leq n$ we get

$$\begin{aligned}\pi(n_1 + \ldots + n_K = n \mid r, p) &= (1-p)^{rK} p^{n-K} \frac{\Gamma(rK + n - K)}{\Gamma(rK)\Gamma(n - K + 1)} \\ &= \begin{cases} \dfrac{(1-p)^{rK} p^{n-K}}{(n-K)B(rK, n-K)} & K < n \\ (1-p)^{rn} & K = n \end{cases}\end{aligned}$$

where $B(\cdot, \cdot)$ is the beta function. This gives the normalising constant of the conditional EPPF and the conditional distribution on the number of clusters $K$.

Integrating out $p$ from the above expression, we get

$$\begin{aligned}\pi(n_1 + \ldots + n_K = n \mid r) &= B(n - K + u, rK + v) \frac{\Gamma(rK + n - K)}{\Gamma(rK)\Gamma(n - K + 1)} \\ &= \frac{\Gamma(n - K + u)\Gamma(rK + n - K)\Gamma(rK + v)}{\Gamma(n - K + 1)\Gamma(n - K + rK + u + v)\Gamma(rK)}\end{aligned}$$

We consider 2 cases:

1. When $u = v = 1$, this reduces to

$$\begin{aligned}\pi(n_1 + \ldots + n_K = n \mid r) &= \frac{rK}{(n - K + rK + 1)(n - K + rK)} \\ &= \frac{n - K + 1}{n - K + rK + 1} - \frac{n - K}{n - K + rK} \\ &= \frac{1}{1 + \omega'_K r} - \frac{\mathbf{1}_{\{K<n\}}}{1 + \omega_K r}\end{aligned}$$

where $\omega_K = \dfrac{K}{n - K}$ and $\omega'_K = \dfrac{K}{n - K + 1}$. Then

$$\begin{aligned}\pi(n_1 + \ldots + n_K = n) &= \frac{\sigma^\eta}{\Gamma(\eta)} \int_0^\infty e^{-\sigma r} r^{\eta - 1} [(1 + \omega'_K r)^{-1} - \mathbf{1}_{\{K<n\}}(1 + \omega_K r)^{-1}] dr \\ &= \sigma^\eta [\omega'^{-\eta}_K U(\eta, \eta, \sigma/\omega'_K) - \mathbf{1}_{\{K<n\}} \omega_K^{-\eta} U(\eta, \eta, \sigma/\omega_K)]\end{aligned}$$

where $U(\cdot, \cdot, \cdot)$ is the confluent hypergeometric function of the second kind and the second equality follows from the integral representation of $U(\cdot, \cdot, \cdot)$; for details see (Gradshteyn and Ryzhik, 2007, p. 1023).

2. When $u$ and $v$ are arbitrary and $\eta > u$ we can use the approximation $\frac{\Gamma(x+a)}{\Gamma(x)} \approx x^a$ to get

$$\pi(n_1 + \ldots + n_K = n \mid r) \approx \frac{\Gamma(n-K+u)}{\Gamma(n-K+1)} \frac{(rK)^v}{(n-K+rK)^{u+v}}$$
$$= \frac{\Gamma(n-K+u)}{\Gamma(n-K+1)} \begin{cases} (rK)^v((n-K)(1+\omega_K r))^{-u-v} & K < n \\ (rK)^{-u} & K = n \end{cases}$$

Then for $K < n$

$$\pi(n_1 + \ldots + n_K = n) \approx \frac{\sigma^\eta}{\Gamma(\eta)} \frac{\Gamma(n-K+u)}{\Gamma(n-K+1)} \frac{K^v}{(n-K)^{u+v}} \int_0^\infty e^{-\sigma r} r^{v+\eta-1}(1+\omega_K r)^{-u-v} dr$$
$$= \frac{\sigma^\eta \Gamma(\eta+v)}{\Gamma(\eta)} \frac{\Gamma(n-K+u)}{\Gamma(n-K+1)} \frac{K^v}{(n-K)^{u+v}} \omega_K^{-(v+\eta)} U(v+\eta, \eta-u+1, \sigma/\omega_K)$$
$$= \frac{\sigma^\eta \Gamma(\eta+v)}{\Gamma(\eta)} \frac{\Gamma(n-K+u)}{\Gamma(n-K+1)} K^{-\eta}(n-K)^{\eta-u} U(v+\eta, \eta-u+1, \sigma/\omega_K)$$

where the second equality follows from the integral representation of $U(\cdot,\cdot,\cdot)$ ((Gradshteyn and Ryzhik, 2007, p. 1023)). For $K = n$

$$\pi(n_1 + \ldots + n_K = n) \approx \frac{\sigma^\eta}{\Gamma(\eta)} \frac{\Gamma(n-K+u)}{\Gamma(n-K+1)} K^{-u} \int_0^\infty e^{-\sigma r} r^{\eta-u-1} dr$$
$$= \frac{\sigma^u \Gamma(u)\Gamma(\eta-u)}{\Gamma(\eta)} n^{-u}$$

# 2 Posterior inference

In this section we provide additional details on the MCMC algorithm used for posterior inference. Recall that we set $\nu = \text{NegBin}(r, p) + 1$ in the ESC model, i.e.,

$$\nu(n_j) = \frac{\Gamma(n_j - 1 + r) p^{n_j - 1}(1-p)^r}{\Gamma(r)(n_j - 1)!}$$

The corresponding conditional EPPF can be calculated from Equation (3) from the main text.

$$\pi(\rho_n \mid r, p) \propto K! p^{n-K}(1-p)^{rK} \prod_{j=1}^{K} n_j \frac{\Gamma(n_j - 1 + r)}{\Gamma(r)} \tag{1}$$

We note that $r$ and $p$ are conditionally independent of the dissimilarities. Therefore, combining Equation (1) with a Gamma$(\eta, \sigma)$ prior for $r$ yields the posterior conditional

distribution for $r$:

$$\pi(r \mid p, \rho_n) \propto r^{\eta-1} \left( \frac{(1-p)^r}{\Gamma(r)} \right)^K \exp(-r\sigma) \prod_{j=1}^{K} \Gamma(n_j - 1 + r) \tag{2}$$

Combining Equation (1) with the Beta$(u, v)$ prior for $p$ yields the posterior conditional distribution for $p$:

$$p \mid \rho_n, r \sim \text{Beta}(n - K + u, rK + v) \tag{3}$$

Conditional reallocation probabilities for the ESC model are computed using Equation (5) from the main text:

$$\pi(z_i = j \mid \mathbf{z}_{-i}, r, p) \propto \begin{cases} (n_{j,-i} + 1) \dfrac{p(n_{j,-i} - 1 + r)}{n_{j,-i}} & j = 1, \ldots, K_{-i} \\ (K_{-i} + 1)(1-p)^r & j = K_{-i} + 1 \end{cases} \tag{4}$$

Let $\boldsymbol{D}$ denote the matrix of all pairwise dissimilarities among the observations in $\boldsymbol{X}$, let $\boldsymbol{D}_{-i}$ denote the set of pairwise dissimilarities in $\boldsymbol{X} \setminus \{x_i\}$, and let $\boldsymbol{D}_i$ denote the set of dissimilarities of $x_i$ from the rest of the observations in $\boldsymbol{X}$. In the following calculations we implicitly condition on $r$ and $p$:

$$\begin{aligned} \pi(z_i = k \mid \boldsymbol{z}_{-i}, \boldsymbol{D}) &= \frac{\pi(z_i = k, \boldsymbol{z}_{-i}, \boldsymbol{D})}{\pi(\boldsymbol{z}_{-i}, \boldsymbol{D})} \\ &= \frac{\pi(z_i = k, \boldsymbol{z}_{-i}, \boldsymbol{D}_{-i})}{\pi(\boldsymbol{z}_{-i}, \boldsymbol{D}_{-i})} \frac{\pi(\boldsymbol{D}_i \mid z_i = k, \boldsymbol{z}_{-i}, \boldsymbol{D}_{-i})}{\pi(\boldsymbol{D}_i \mid \boldsymbol{z}_{-i}, \boldsymbol{D}_{-i})} \\ &= \frac{\pi(z_i = k \mid \boldsymbol{z}_{-i})}{\pi(\boldsymbol{D}_i \mid \boldsymbol{z}_{-i}, \boldsymbol{D}_{-i})} \int \pi(\boldsymbol{D}_i \mid z_i = k, \boldsymbol{z}_{-i}, \boldsymbol{D}_{-i}, \boldsymbol{\lambda}, \boldsymbol{\theta}) \; d\pi_\lambda \; d\pi_\theta \end{aligned}$$

In the last expression, the ratio $\dfrac{\pi(z_i = k, \boldsymbol{z}_{-i}, \boldsymbol{D}_{-i})}{\pi(\boldsymbol{z}_{-i}, \boldsymbol{D}_{-i})}$ has been reduced to $\pi(z_i = k \mid \boldsymbol{z}_{-i})$ using the conditional independence of $\boldsymbol{D}_{-i}$ and $z_i$ given $\boldsymbol{z}_{-i}, r$, and $p$. The quantity $\dfrac{1}{\pi(\boldsymbol{D}_i \mid \boldsymbol{z}_{-i}, \boldsymbol{D}_{-i})}$ does not depend on $k$ and can be factored out. The integrand is

$$\begin{aligned} \pi(\boldsymbol{D}_i \mid z_i = k, \boldsymbol{z}_{-i}, \boldsymbol{D}_{-i}, \boldsymbol{\lambda}, \boldsymbol{\theta}) = &\left[ \prod_{j \in C_{k,-i}} \frac{d(x_i, x_j)^{\delta_1 - 1} \lambda_k^{\delta_1}}{\Gamma(\delta_1)} \exp(-\lambda_k d(x_i, x_j)) \right] \times \\ &\left[ \prod_{\substack{t=1 \\ t \neq k}}^{K_{-i}} \prod_{j \in C_{t,-i}} \frac{d(x_i, x_j)^{\delta_2 - 1} \theta_{kt}^{\delta_2}}{\Gamma(\delta_2)} \exp\left(-\theta_{kt} d(x_i, x_j)\right) \right] \end{aligned}$$

A straightforward computation of the integral then gives

$$\pi(z_i = k \mid \boldsymbol{z}_{-i}, \boldsymbol{D}, r, p) \propto \begin{cases} (n_{k,-i}+1)\dfrac{p(n_{k,-i}-1+r)}{n_{k,-i}}\mathcal{L}_{ik}^{(1)}\mathcal{L}_{ik}^{(2)} & k = 1, \dots, K_{-i} \\ (K_{-i}+1)(1-p)^r \mathcal{L}_{ik}^{(2)} & k = K_{-i}+1 \end{cases} \tag{5}$$

where

$$\mathcal{L}_{ik}^{(1)} = \frac{\Gamma(\alpha_{ik})\beta^{\alpha}}{\Gamma(\alpha)\beta_{ik}^{\alpha_{ik}}} \prod_{j \in C_{k,-i}} \frac{D_{ij}^{\delta_1 - 1}}{\Gamma(\delta_1)}, \qquad \alpha_{ik} = \alpha + \delta_1 n_{k,-i}, \qquad \beta_{ik} = \beta + \sum_{j \in C_{k,-i}} D_{ij}$$

$$\mathcal{L}_{ik}^{(2)} = \prod_{\substack{t=1 \\ t \neq k}}^{K_{-i}} \frac{\Gamma(\zeta_{it})\gamma^{\zeta}}{\Gamma(\zeta)\gamma_{it}^{\zeta_{it}}} \prod_{j \in C_{t,-i}} \frac{D_{ij}^{\delta_2 - 1}}{\Gamma(\delta_2)}, \qquad \zeta_{it} = \zeta + \delta_2 n_{t,-i}, \qquad \gamma_{it} = \gamma + \sum_{j \in C_{t,-i}} D_{ij}$$

## 2.1 MCMC Algorithm

1. Sample $r$ from its posterior full conditional in Equation (2). We perform a random walk Metropolis step, using a $[0, \infty)$-truncated Normal distribution centred at the current value as the proposal. This step can be adapted if required, for example with slice sampling (Neal (2003)) as suggested by Betancourt *et al.* (2022).

2. Sample $p$ from its posterior full conditional in Equation (3).

3. The cluster allocation labels $z_i$ can be sampled through either a Gibbs-style algorithm or a split-and-merge scheme (Jain and Neal, 2004). For the Gibbs step, sample each $z_i$ from its full conditional in Equation (5). For the split-merge scheme, which is a Metropolis-Hastings step, we follow section 3.3.2 of Jain and Neal (2004). In this case, the prior ratio for the Metropolis-Hastings acceptance ratio in the split step can be calculated from Equation (1), and is given by

$$\frac{\pi(\boldsymbol{z}_{\text{split}} \mid r, p)}{\pi(\boldsymbol{z} \mid r, p)} = \frac{(K+1)(1-p)^r n_i' n_j' \Gamma(n_i' + r - 1)\Gamma(n_j' + r - 1)}{p n_i \Gamma(r)\Gamma(n_i + r - 1)} \tag{6}$$

where $K$ is the current number of clusters, $n_i$ is the size of the cluster that is being split, and $n_i'$ and $n_j'$ are the sizes of the clusters that it is split into. Similarly the prior ratio for the merge step is given by

$$\frac{\pi(\boldsymbol{z}_{\text{merge}} \mid r, p)}{\pi(\boldsymbol{z} \mid r, p)} = \frac{p\Gamma(r)(n_i + n_j)\Gamma(n_i + n_j + r - 1)}{K(1-p)^r n_i n_j \Gamma(n_i + r - 1)\Gamma(n_j + r - 1)} \tag{7}$$

where $n_i$ and $n_j$ are the sizes of the clusters being merged. Following the recommendations of section 3.4 of Jain and Neal (2004), we alternate between Metropolis-Hastings updates and full Gibbs updates of the cluster labels.

Note that we do not sample the $\lambda_k$ and $\theta_{kt}$ as we marginalise over them. If required, they can be sampled by conditioning on the cluster allocation and sampling from a Gamma-Gamma conjugate model.

## 2.2 Computational Cost

In our implementation, each Gibbs update of cluster labels has a worst case complexity of $O(n^2)$, and the update of a single cluster label $z_i$ requires $O(n + K_{-i})$ operations. While reallocating $z_i$, we pre-compute the quantities $\alpha_{ik}, \beta_{ik}, \zeta_{ik}$, $\gamma_{ik}$, and $\prod_{j \in C_{k,-i}} D_{ij}$ for each $k$ in $1, \ldots, K_{-i}$. For fixed $k$, the computation of $\beta_{ik}$, $\gamma_{ik}$, and $\prod_{j \in C_{k,-i}} D_{ij}$ each requires $n_{k,-i}$ operations, while each of the remaining quantities can be computed in a single operation. Therefore the pre-computation step takes $n - 1$ operations. With this pre-computation the calculation of $\mathcal{L}_{ik}^{(1)}$ takes a single operation for each $k$. We also pre-compute an auxilliary quantity

$$\mathcal{L}_{it}^{(3)} = \frac{\Gamma(\zeta_{it})\gamma^{\zeta}}{\Gamma(\zeta)\gamma_{it}^{\zeta_{it}}} \prod_{j \in C_{t,-i}} \frac{D_{ij}^{\delta_2 - 1}}{\Gamma(\delta_2)}$$

for each $t$ in $1, \ldots, K_{-i}$. The difference between $\mathcal{L}_{ik}^{(3)}$ with $\mathcal{L}_{ik}^{(2)}$ is that $t$ also takes the value $k$ in the first product in the expression for $\mathcal{L}_{ik}^{(3)}$. The computation of $\mathcal{L}_{ik}^{(3)}$ takes $K_{-i}$ operations. Then

$$\mathcal{L}_{ik}^{(2)} = \begin{cases} \prod_{t=1}^{K_{-i}} \mathcal{L}_{it}^{(3)} \Big/ \mathcal{L}_{ik}^{(3)} & k = 1, \ldots, K_{-i} \\ \prod_{t=1}^{K_{-i}} \mathcal{L}_{it}^{(3)} & k = K_{-i} + 1 \end{cases}$$

so $\mathcal{L}_{ik}^{(2)}$ can be computed for each $k$ in a single operation. Together the above computations give $O(n + K_{-i})$ operations for the reallocation of $z_i$ as claimed. Since $K_{-i} \leq n$, we get a complexity of $O(n^2)$ for each full Gibbs update.

Each split-merge iteration also has a worst-case complexity of $O(n^2)$. This is because it comprises a series of restricted Gibbs scans and the computation of the acceptance ratio. The acceptance ratio comprises a prior ratio, which can be computed in a single operation; a proposal ratio, which can be computed alongside the Gibbs scans; and a likelihood ratio. A naive calculation of the likelihood requires $\sum_{k,t=1}^{K} n_k n_t \leq n^2$ operations. Thus the acceptance ratio takes at most $O(n^2)$ operations to compute.

We note that the precomputation steps above as well as the subsequent computation of $\mathcal{L}_{ik}^{(1)}$ and $\mathcal{L}_{ik}^{(2)}$ are amenable to vectorization.

# 3 Numismatic Example

## 3.1 Pre-processing

The appearance of an ancient coin is usually unique because no two blank coins were ever struck at exactly the same angle or with the same force and dies deteriorated over the course of the minting process, resulting in different impressions. Other factors influencing variation in coin appearance include coin blank material, craftsmanship, tools used in minting, the specific die, mint signs and shape. Furthermore, coins suffered from wear and tear, were clipped to shave off precious metal, or were marked by money changers and government authorities. As a result, specimens struck from the same die may show a large degree of variability, whereas coins of the same type may look very similar, even when struck from different dies, because all dies of the same issue were based on a common prototype. In addition to the variations in the physical appearance of the coins, their images vary considerably in overall quality, in size, and in lighting conditions during image acquisition; ranging from high-resolution colour images to halftone images. Before defining dissimilarity measures and distances between coins, the following pre-processing steps were therefore applied to all images. After converting all images to greyscale and resizing them to the mode of the image sizes in the dataset, total-variation image restoration (Rudin *et al.*, 1992) is performed on each image to reduce noise introduced during image acquisition, e.g. as result of low lighting, as well as to even out small aberrations, while preserving the quality of edges and corners in the images. Contrast limited adaptive histogram equalisation (Pizer *et al.*, 1987) is then applied to locally enhance contrast and edge definitions, while limiting noise amplification in near-constant image regions. Potential artefacts introduced by the local transformations used in the latter procedure are then reduced by a second application of total-variation restoration.

## 3.2 Computing pairwise dissimilarities

SIFT is used to calculate for each image (1) a number of keypoints, to which we refer as landmarks, (2) associated descriptor vectors containing local gradient information from a neighbourhood of the respective landmark, and (3) a weighted average of the local gradient orientations around the respective landmark. Given an image pair $(i, j)$, each landmark of image $i$ is then associated with its best matching landmark in image $j$ according to the similarity of their descriptor vectors (see (Lowe, 2004, Section 7.1)), resulting in a subset of matched landmarks between the images $i$ and $j$. In general, not every landmark in image $i$ is associated to a landmark in image $j$, and unmatched landmarks, arising for example from noise or artefacts present in only one of the two images, are discarded. In order to increase the geometric consistency of the pre-selected landmark matches provided by SIFT, the number of matched landmark pairs is then further reduced using the low-distortion correspondence

filtering of Lipman *et al.* (2014), resulting in the largest subset of the pre-selected matched landmarks that can be aligned using a non-rigid deformation that keeps global distortion below a specified bound.

Initial experiments indicate that the total number of matched landmarks remaining after low-distortion filtering, together with their Procrustes distance (i.e. the minimal total Euclidean energy between the matched landmarks over all possible rigid motions between the two landmark sets, see Gower 1975 and Gower *et al.* 2004), already has considerable potential to construct a dissimilarity measure on the basis of which to discriminate between pairs of coins minted from the same die and from different dies. We combine these with additional metrics calculated for the matched landmarks from their SIFT descriptor vectors and average local gradient orientations to further aid discrimination. In the definitions of these additional metrics, which we describe below, we take into account the relative importance of individual matched landmark pairs by ranking them according to an adaptation of the reweighted Gaussian Process method for selecting landmarks on anatomical surfaces introduced by Gao *et al.* (2019). This method uses a Gaussian Process with variance-covariance structure altered by reweighting its radial-basis-function kernels to incorporate geometrically or semantically meaningful information. In their original work, Gao *et al.* (2019) select landmarks from a discrete set of points on a single anatomical surface. We extend their method from ranking landmarks to ranking matched pairs of landmarks by assuming a Gaussian Process on the space of paired pixel positions. The algorithm then ranks the existing landmark pairs through a greedy process, successively picking as a new landmark pair the candidate with largest conditional prediction variance conditioned on the previously selected landmark pairs. In our application we reweight the variance-covariance matrix using weights defined as the product of two factors. The first factor is the average Euclidean distance of the individual landmarks of each pair to the closest landmark in its respective image, while the second factor is the Euclidean distance of the descriptor vectors of the landmarks of the matched pair. While the first factor emphasizes matched pairs whose discriminative potential stems from the fact that they are spatially isolated in the two coins, the second factor emphasizes matched pairs whose respective neighbourhoods are topologically different. Once the landmark pairs are ranked, we assign to the top ten pairs a weight of $1/m$ where $m$ is the rank, while we prefer to assign a constant weight $1/10$ to the remaining pairs as the ranking procedure is less stable.

To finally define a dissimilarity between images, we compute the following metrics

1. the number of low distortion landmark matches for the given image pair;
2. the Procrustes distance of these matched landmark sets;
3. the minimum pairwise Euclidean distance over all rank-reweighted SIFT descriptor vectors between the matched landmarks;

4. the log-transformed minimum pairwise difference of the rank-reweighted local gradient orientation between matched landmarks of the coin pair;

5. the log-transformed rank-reweighted average of the differences of all local gradient orientations.

Although more dissimilarity metrics are available, we find metrics (1)-(5) to be the most discriminating between images of coins from different dies. Note that different sets of coins besides the Nero set are available to our group, and have been used to draw these conclusions. The dissimilarity measures (1)-(5) are combined to a vector whose Euclidean norm serves as a dissimilarity score for the image pair.

Finally, we observe that the above procedure produces some image pairs with zero matched landmarks and infinite dissimilarity, and other image pairs with perfectly matched landmark pairs and zero dissimilarity (the latter is most common with slightly different images of the same coin). For the pairs with infinite no matched landmarks, we set their dissimilarity to 0.9 times the maximum finite dissimilarity in our dataset. For the image pairs with perfectly matched landmarks, we set their dissimilarity to 1.1 times the minimum nonzero dissimilarity in our dataset.

## 3.3 Additional Figures for the Numismatic Example

Here we provide additional figures and results for the numismatic example. Figure 1 shows the comparison between the prior predictive distribution of within-cluster and inter-cluster dissimilarities to the kernel density estimates from the data. Figure 2 shows the posterior distributions for $r$ and $p$. Figure 3 shows the coclustering matrices for the various clustering point estimates obtained as detailed in the main paper.

Table 1 gives the integrated autocorrelation coefficient (IAC), effective sample size (ESS), and effective sample size divided by the number of samples (i.e. the effective sample rate or ESR). In Figure 4 we show the plots of the autocorrelation function for $K$, $r$, and $p$ for lags from zero to $10\log_{10}(\text{number of samples}) = 46$. Figure 5 shows the trace-plot of log-likelihood. These diagnostics show satisfactory mixing and convergence of the chains.

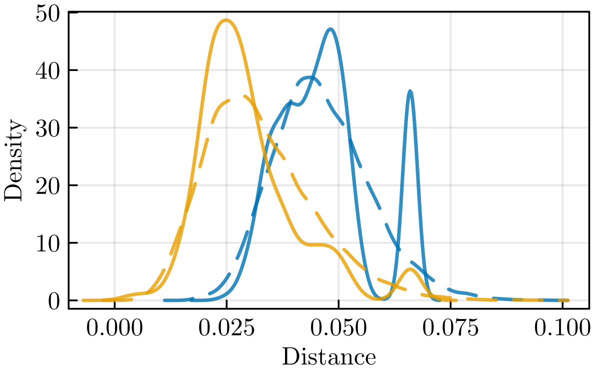


Figure 1. Coins data: Predictive prior distribution (dashed lines) of the within-cluster dissimilarities (orange) and inter-cluster dissimilarities (blue) overlaid with the kernel density estimate of the true dissimilarities (solid lines).

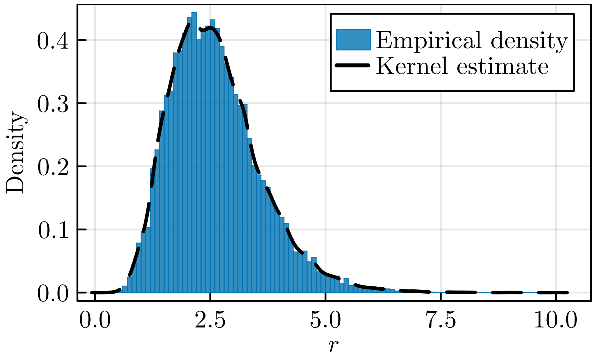


(a) $r$

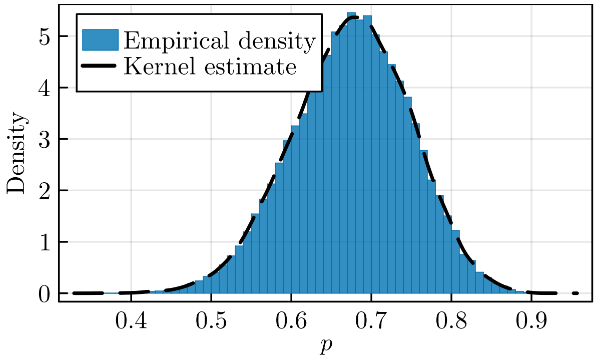


(b) $p$

Figure 2. Coins data: Distribution of posterior samples of $r$ and $p$

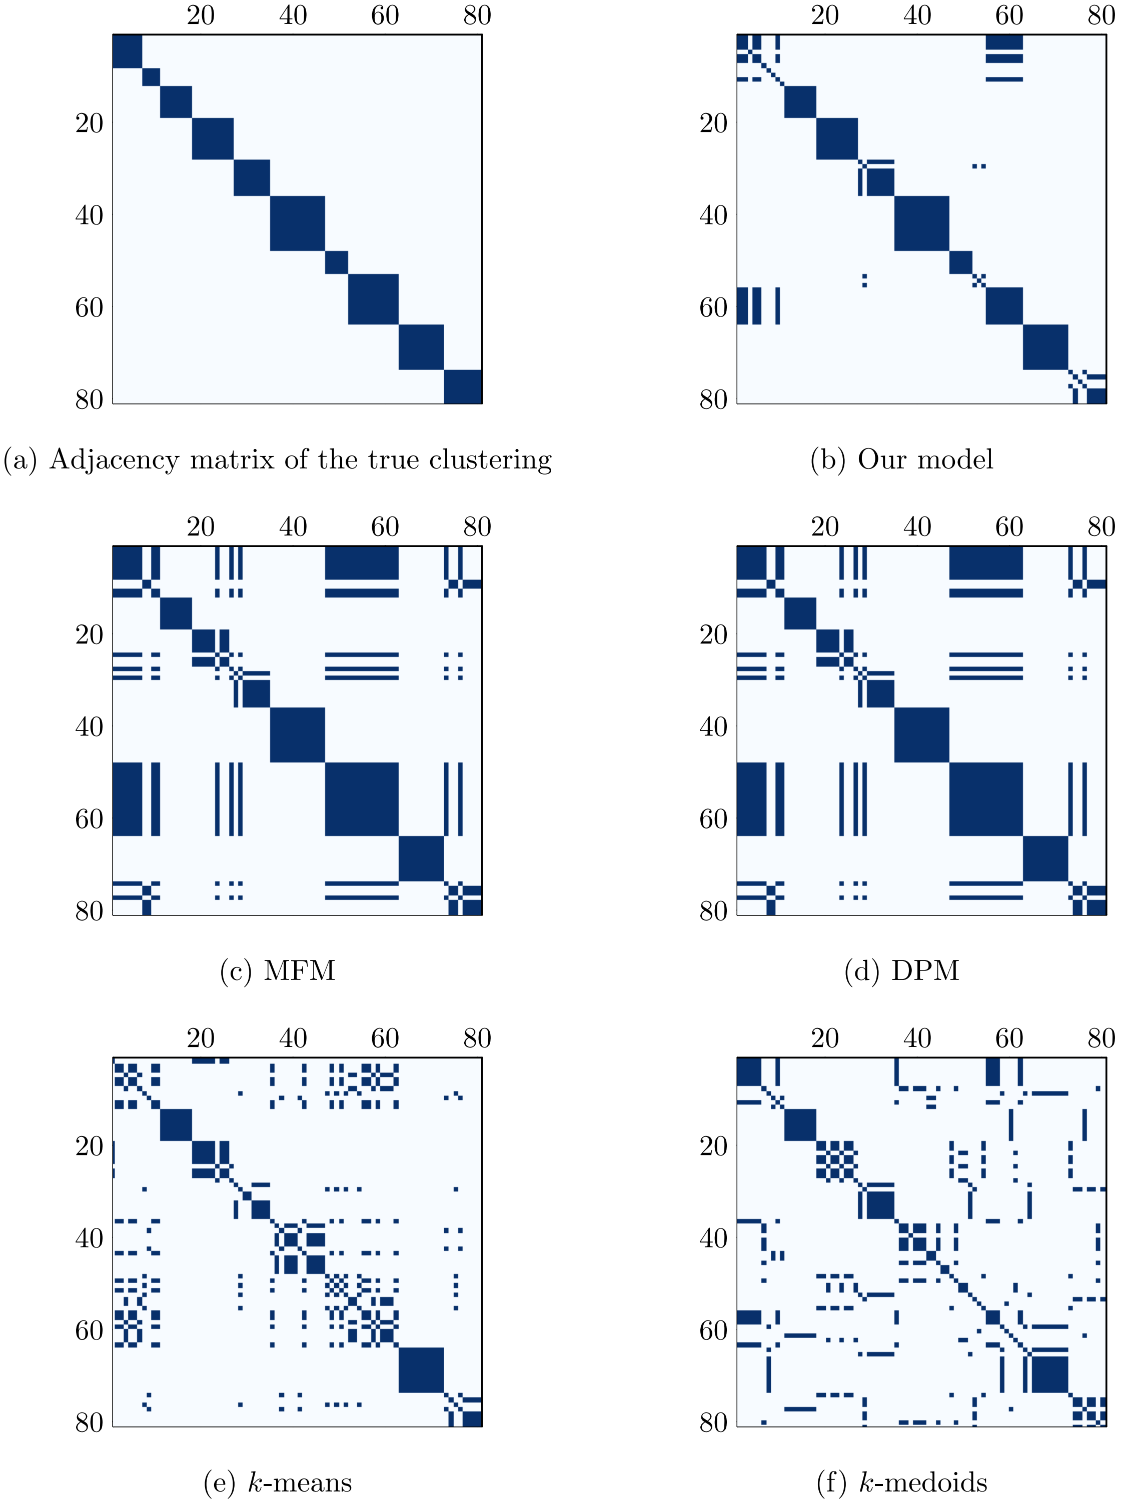


(a) Adjacency matrix of the true clustering

(b) Our model

(c) MFM

(d) DPM

(e) $k$-means

(f) $k$-medoids

Figure 3. Coins data: adjacency matrices of the point estimates

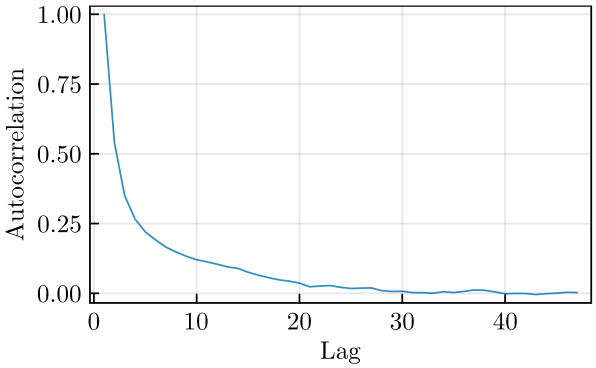


(a) $K$

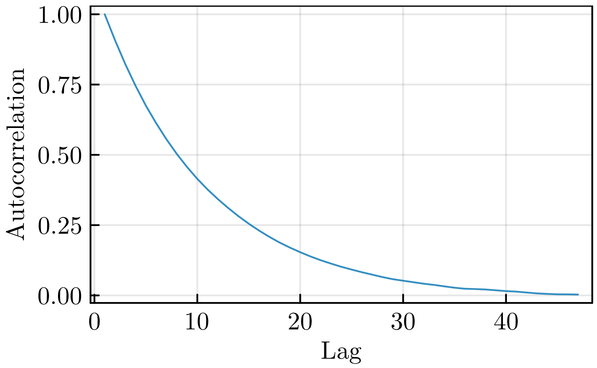


(b) $r$

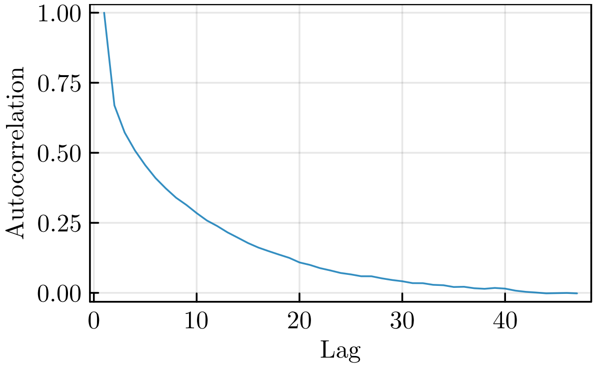


(c) $p$

Figure 4. Coins data: Autocorrelation plots for $K$, $r$, and $p$

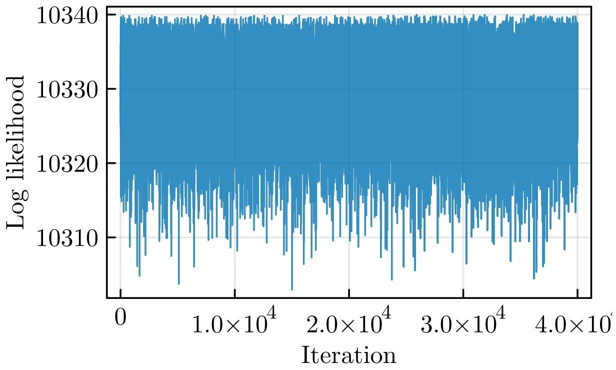


Figure 5. Coins data: Log-likelihood trace-plot

| | IAC | ESS | ESR |
|---|---|---|---|
| K | 8.17 | 4894.37 | 0.12 |
| r | 20.89 | 1914.56 | 0.05 |
| p | 15.20 | 2632.37 | 0.07 |

Table 1. Coins example: Convergence Diagnostics

# 4 Simulation Studies

We generate 100 points from a mixture of ten multivariate Normal kernels with cluster centres at the vertices of the standard $d$-simplex and covariance matrices $\sigma^2 I_d$. We run three experiements, with $(\sigma, d) \in \{(0.25, 10), (0.2, 50), (0.18, 10)\}$. Cluster weights are drawn from a Dirichlet prior with $\alpha = 10$. Figures 6a, 13a and 20a show the histogram of pairwise Euclidean distances. In Figures 6c, 13c and 20c we compare the prior predictive distribution of within-cluster and inter-cluster distances to the kernel density estimates from the data. We also show the implied prior predictive distribution on the number of clusters $K$ in Figures 6b, 13b and 20b. We run the algorithm for 50000 iterations, discarding the first 10000 iterations as burnin. We compare our model to our model without repulsion, MFM, and DPM. In Figures 9, 16 and 23 we compare the (a) the true adjacency matrix and (b) the oracle estimate of the co-clustering matrix to the co-clustering matrices obtained with (c) our model, (d) our model without repulsion, (e) MFM, and (f) DPM. The oracle estimate of the co-clustering matrix is obtained analytically by assuming knowledge of the number of clusters, cluster proportions, as well as the parameters defining the cluster kernels. The MFM and DPM models are fitted on the original data and not on the distances, making full use of the information available. In each case the co-clustering matrix from our model is comparable to the oracle co-clustering matrix, and in general both recover well the true clustering structure. We also show the posterior distribution of the number of clusters $K$ in Figures 7, 14 and 21. We note that the lack of a repulsion in our model leads to a very large number of clusters. This suggests that the repulsion term plays an important role as an identifiability constraint which allows for better cluster estimation. We elaborate on this point in Section 6. We show the posterior distributions on $r$ and $p$ in Figures 8, 15 and 22.

Tables 3, 5 and 7 give the integrated autocorrelation coefficient (IAC), effective sample size (ESS), and effective sample size divided by the number of samples (i.e. the effective sample rate or ESR). In Figures 11, 18 and 25 we show the plots of the autocorrelation function for $K$, $r$, and $p$ for lags from zero to $10 \log_{10}(\text{number of samples}) = 46$. Figures 12, 19 and 26 show the trace-plot of log-likelihood for each experiment. These diagnostics show satisfactory mixing and convergence of the chains.

As in our numismatic example, point estimates are obtained for each method via the SALSO algorithm. Point estimates are also obtained via k-means (on the original data) and k-medoids (on the distances) using the value of $K$ obtained by the elbow method as in Section 2.4.1 of the main paper. These point estimates are compared to the true clustering in Tables 2, 4 and 6. In Figures 10, 17 and 24 we show the adjacency matrices corresponding to the various point-estimates. The findings from these simulation studies are consistent with the results of the numismatic example, confirming that the proposed strategy is effective for clustering in high dimensions.

## 4.1 Simulation Study 1

In our first example we use $\sigma = 0.25$ and $d = 10$. In this example there is significant overlap between the distribution of within-cluster and between-cluster distances, and the clusters are poorly separated.

| | Our Model | MFM | DPM | $k$-means | $k$-medoids |
|---|---|---|---|---|---|
| Binder loss | 0.02 | 0.3 | 0.29 | **0.02** | 0.05 |
| NVI distance | 0.09 | 0.36 | 0.36 | **0.08** | 0.19 |
| ARI | 0.85 | 0.24 | 0.25 | **0.88** | 0.69 |
| NMI | 0.90 | 0.48 | 0.51 | **0.92** | 0.80 |
| K | 15 | 3 | 3 | 12 | 12 |

Table 2. Simulation study 1: Clustering accuracy of point estimates with respect to the true clustering

| | IAC | ESS | ESR |
|---|---|---|---|
| K | 6.57 | 6088.71 | 0.15 |
| r | 18.21 | 2196.56 | 0.05 |
| p | 13.75 | 2908.51 | 0.07 |

Table 3. Simulation study 1: Convergence diagnostics

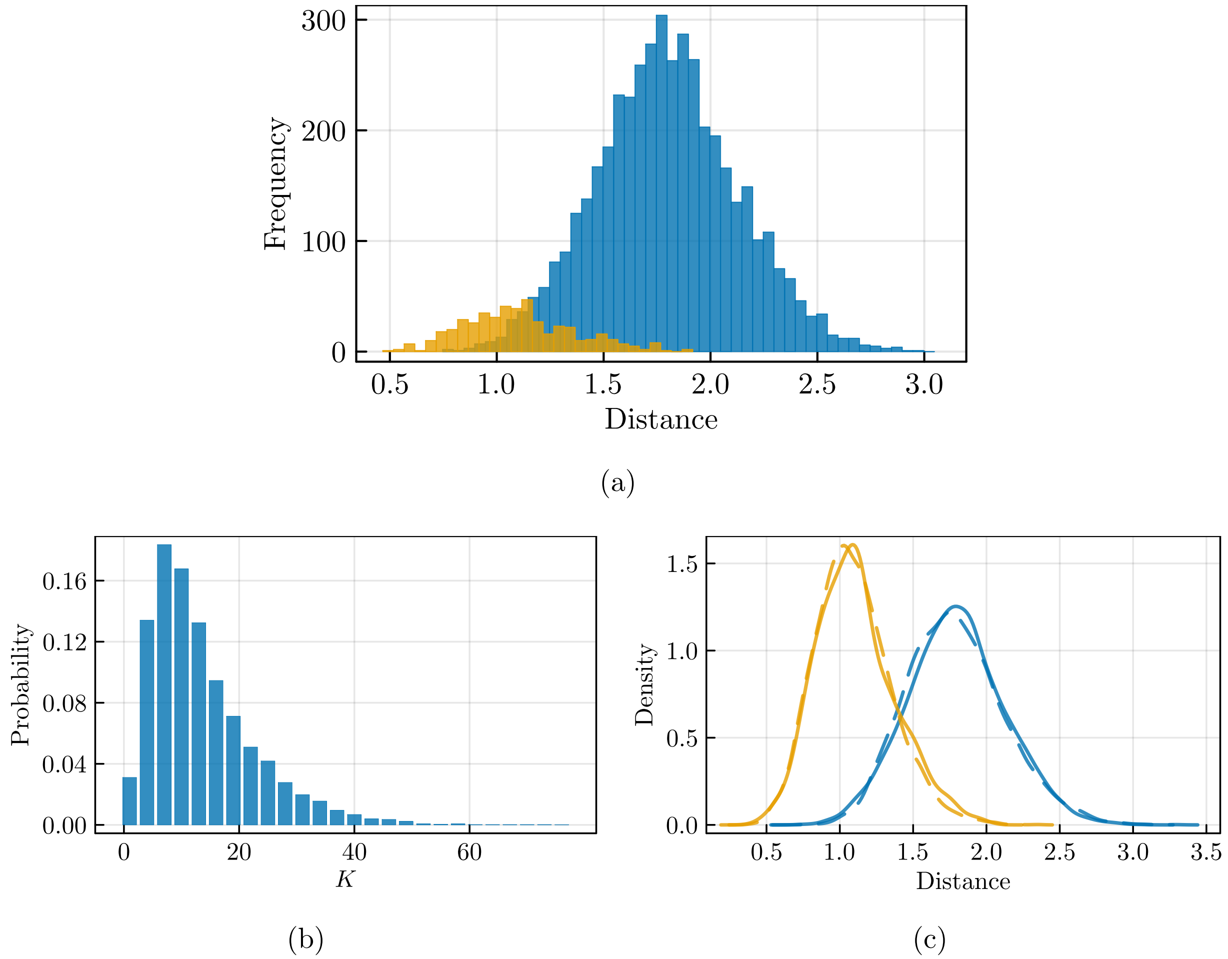


Figure 6. Simulated dataset 1: (a) Histogram of within-cluster distances (orange) and inter-cluster distances (blue). (b) Implied prior on the number of clusters $K$. (c) Predictive prior distribution (dashed lines) of the within-cluster distances (orange) and inter-cluster distances (blue) overlaid with the kernel density estimate of the true distances (solid lines).

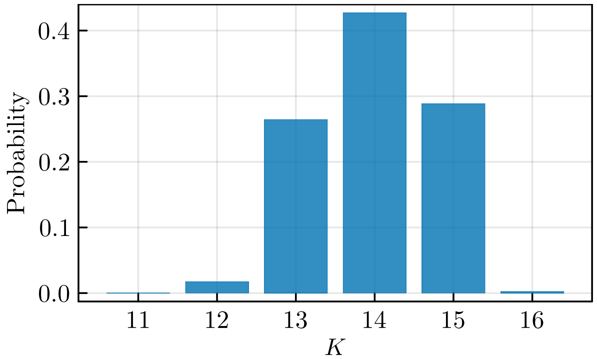


(a) Our model

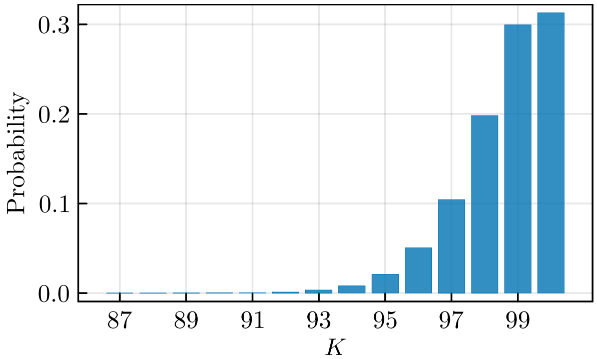


(b) Our model without repulsion

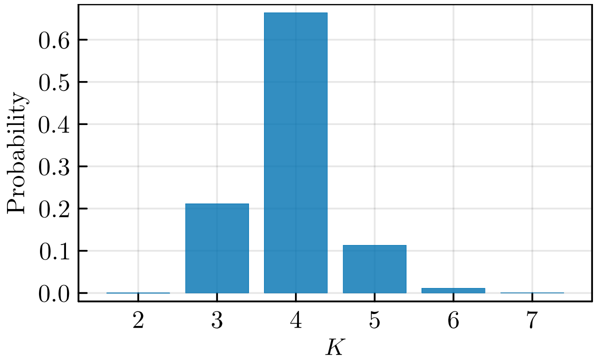


(c) MFM

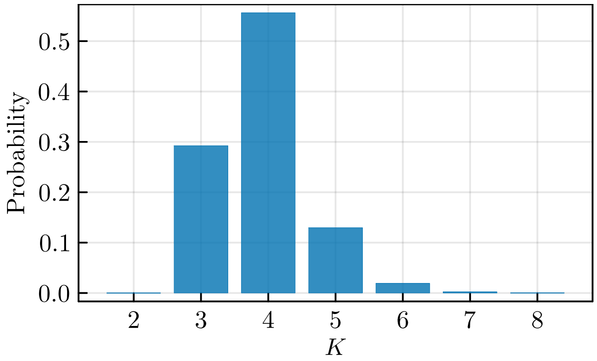


(d) DPM

Figure 7. Simulation study 1: Posterior distribution of the number of clusters $K$

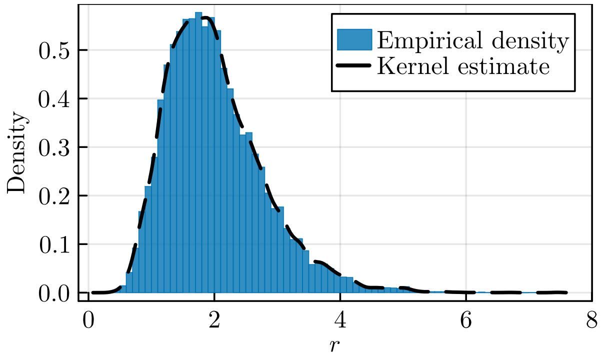


(a) $r$

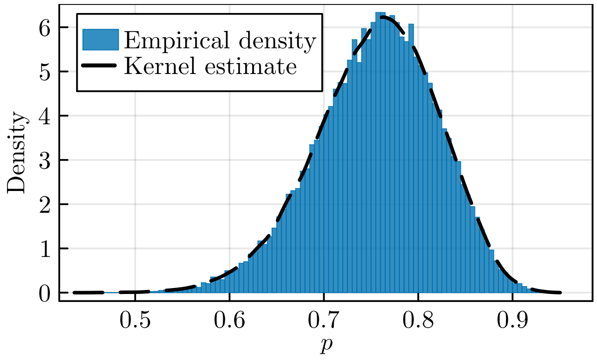


(b) $p$

Figure 8. Simulation study 1: Posterior distribution of $r$ and $p$

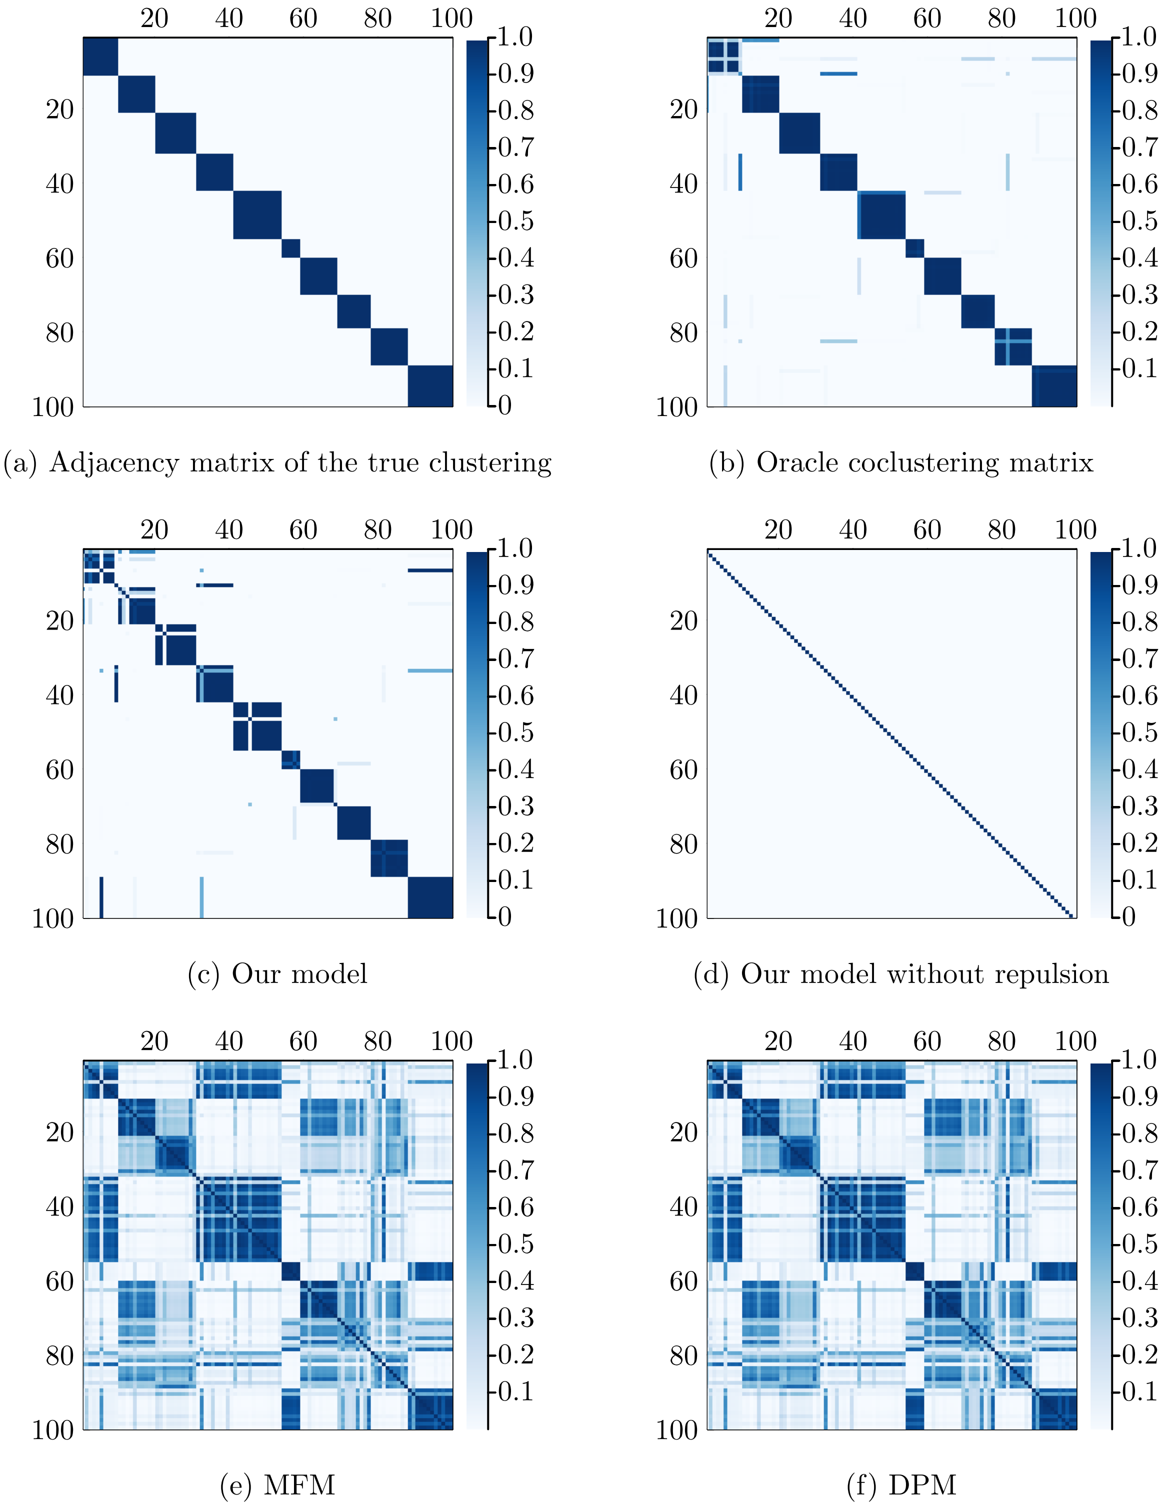


(a) Adjacency matrix of the true clustering

(b) Oracle coclustering matrix

(c) Our model

(d) Our model without repulsion

(e) MFM

(f) DPM

Figure 9. Simulation study 1: Posterior co-clustering matrices

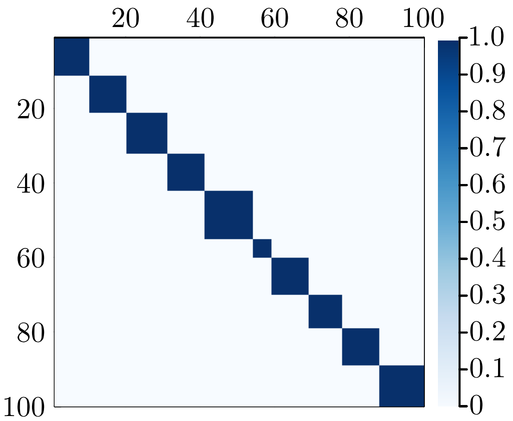


(a) Adjacency matrix of the true clustering

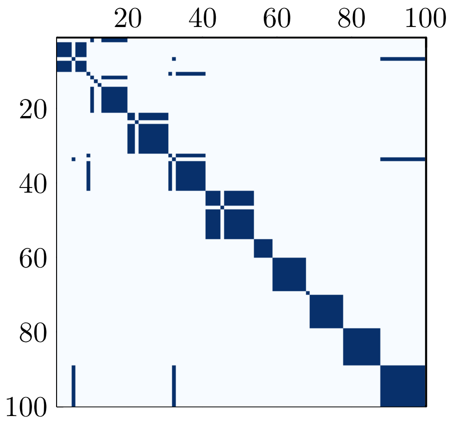


(b) Our model

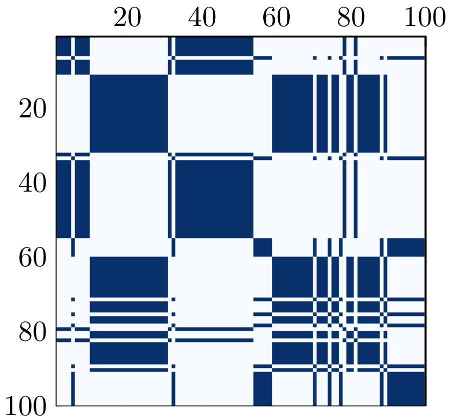


(c) MFM

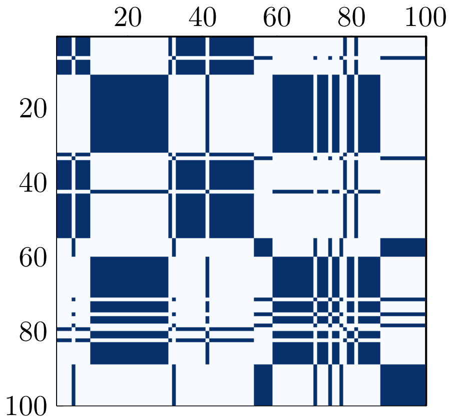


(d) DPM

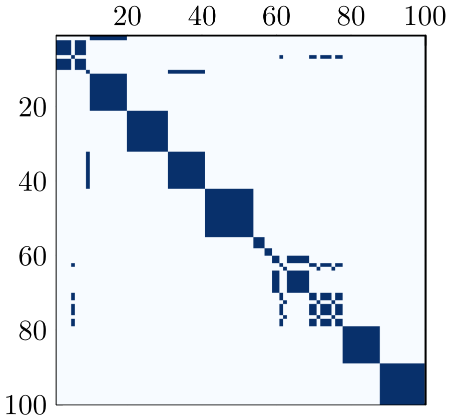


(e) $k$-means

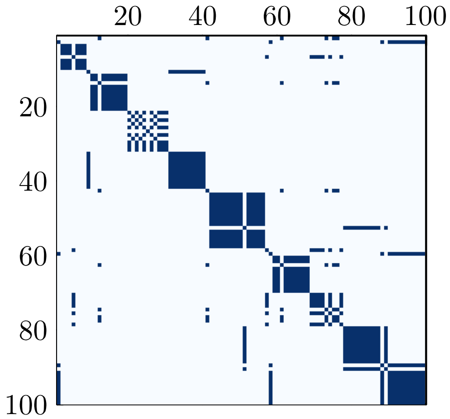


(f) $k$-medoids

Figure 10. Simulation study 1: Adjacency matrices of the point estimates

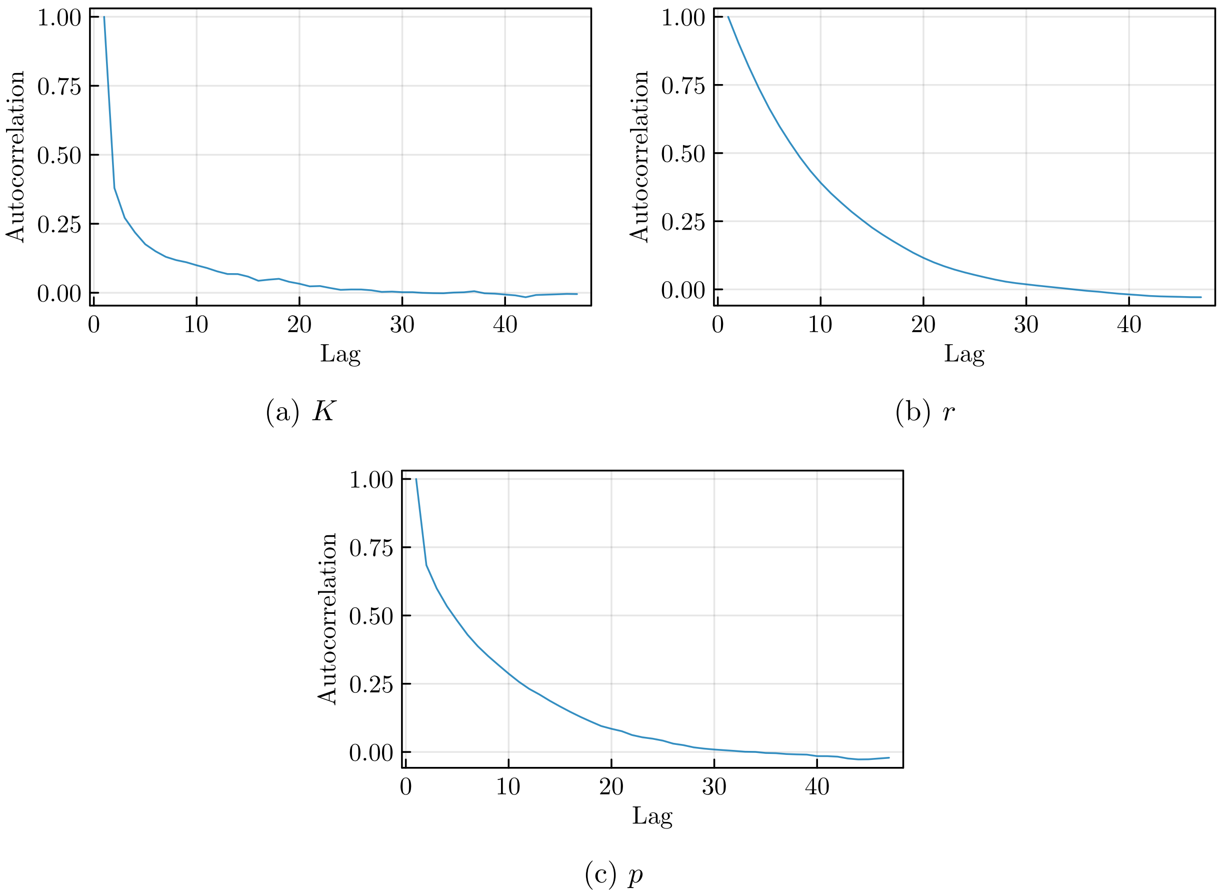


Figure 11. Simulation study 1: Autocorrelation plots for $K$, $r$, and $p$

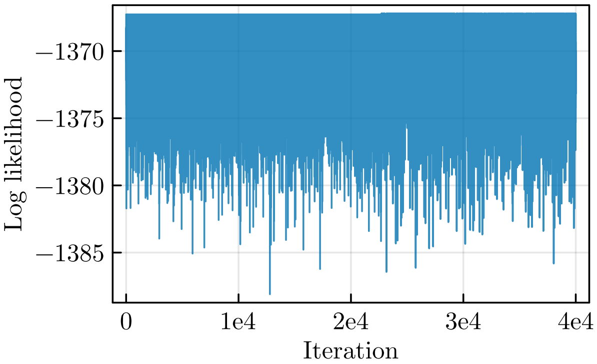


Figure 12. Simulation study 1: Log-likelihood trace-plot

## 4.2 Simulation Study 2: Higher Dimensional Example

Here we consider higher dimensional data generated using $\sigma = 0.2$, $d = 50$ (in the previous example we use $d = 10$). This parameter setting leads to greater overlap between the within-cluster and inter-cluster distances, as seen in Figure 13a. Our model performs well in this scenario too, as evident from Figures 14 and 16 and Table 4.

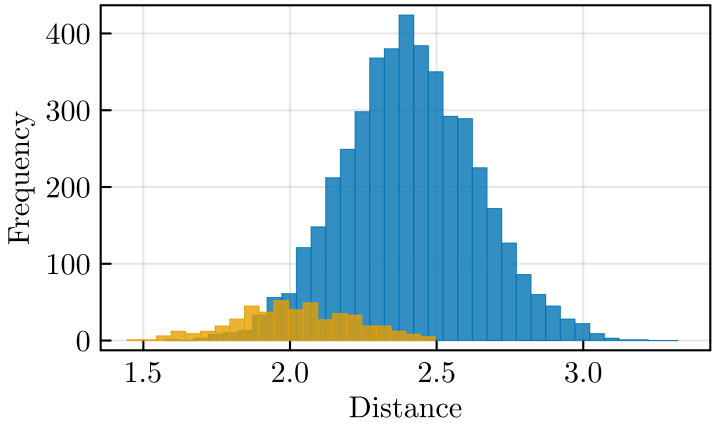


(a)

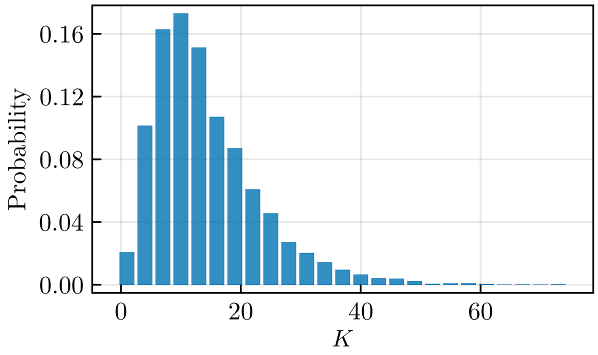


(b)

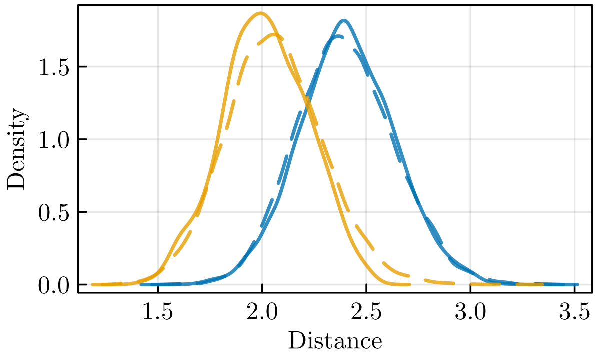


(c)

Figure 13. Simulated dataset 2: (a) Histogram of within-cluster distances (orange) and inter-cluster distances (blue). (b) Implied prior on the number of clusters $K$. (c) Predictive prior distribution (dashed lines) of the within-cluster distances (orange) and inter-cluster distances (blue) overlaid with the kernel density estimate of the true distances (solid lines).

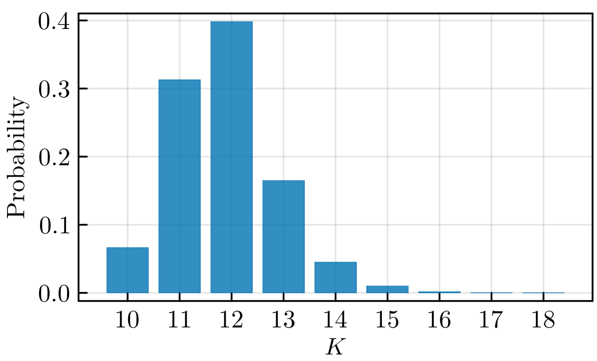


(a) Our model

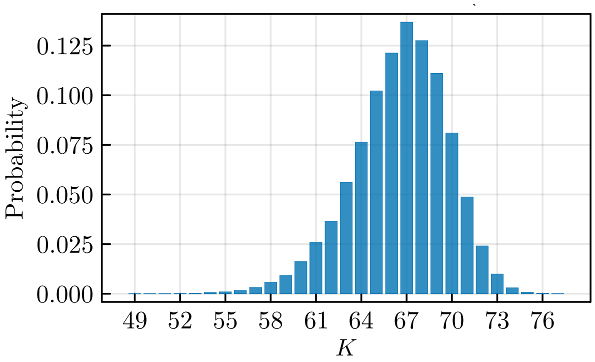


(b) Our model without repulsion

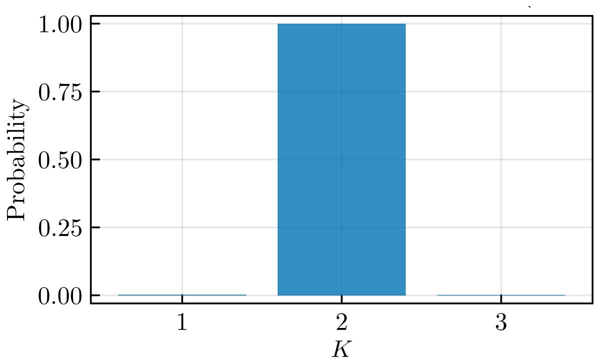


(c) MFM

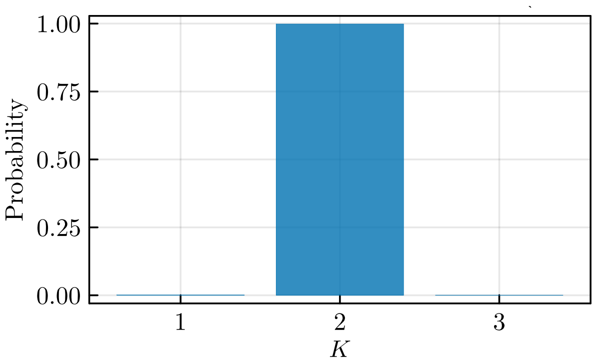


(d) DPM

Figure 14. Simulation study 2: Posterior distribution of the number of clusters $K$

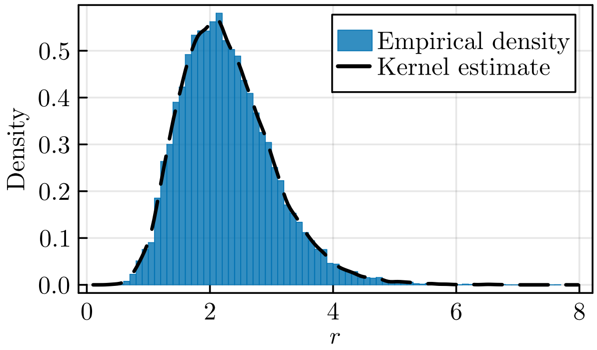


(a) $r$

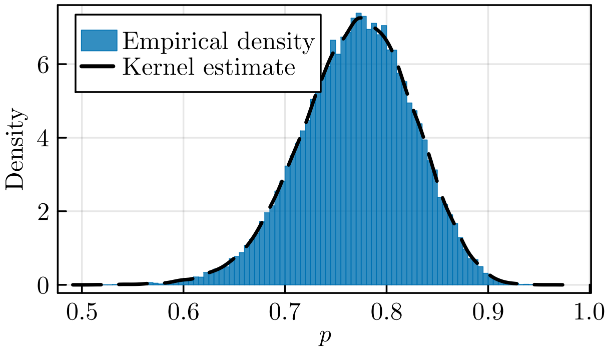


(b) $p$

Figure 15. Simulation study 2: Posterior distribution of $r$ and $p$

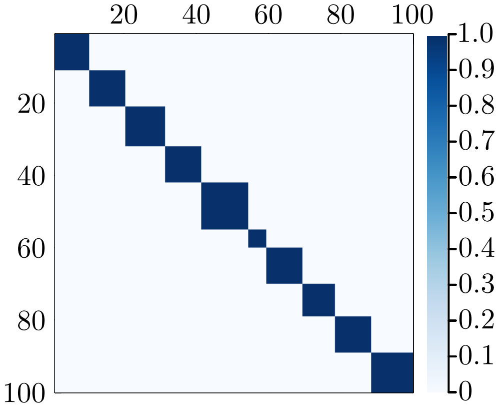


(a) Adjacency matrix of the true clustering

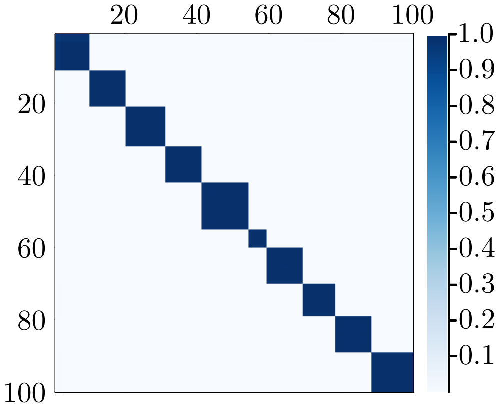


(b) Oracle coclustering matrix

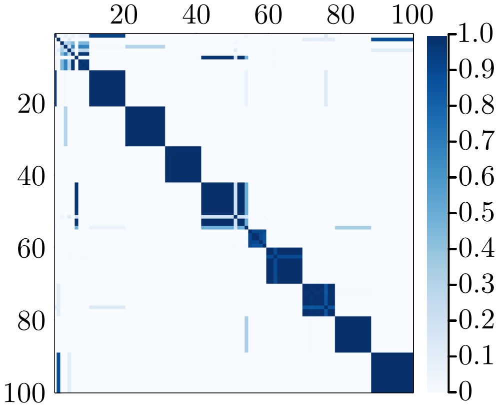


(c) Our model

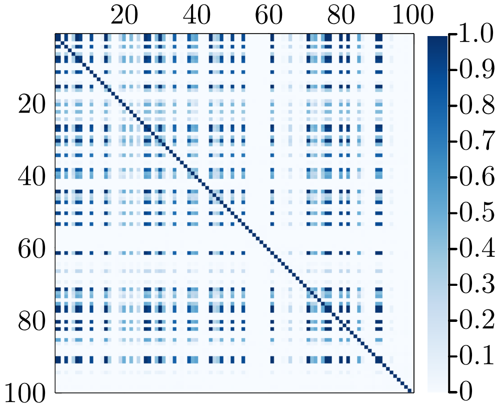


(d) Our model without repulsion

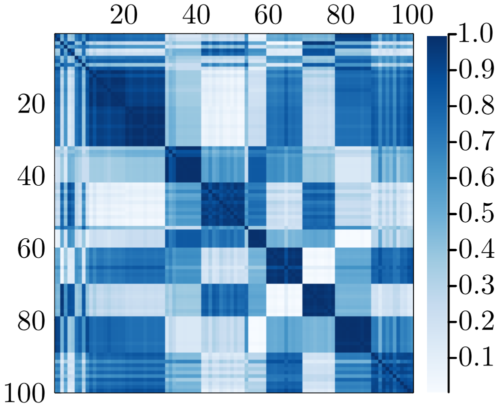


(e) MFM

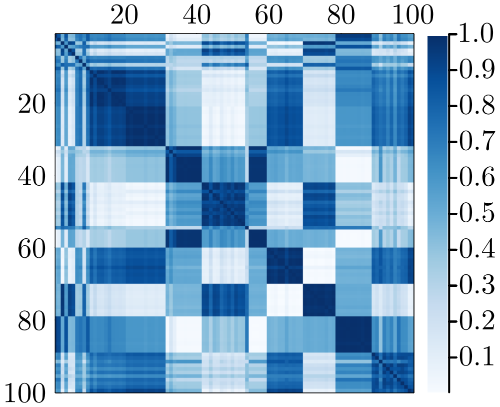


(f) DPM

Figure 16. Simulation study 2: Posterior co-clustering matrices

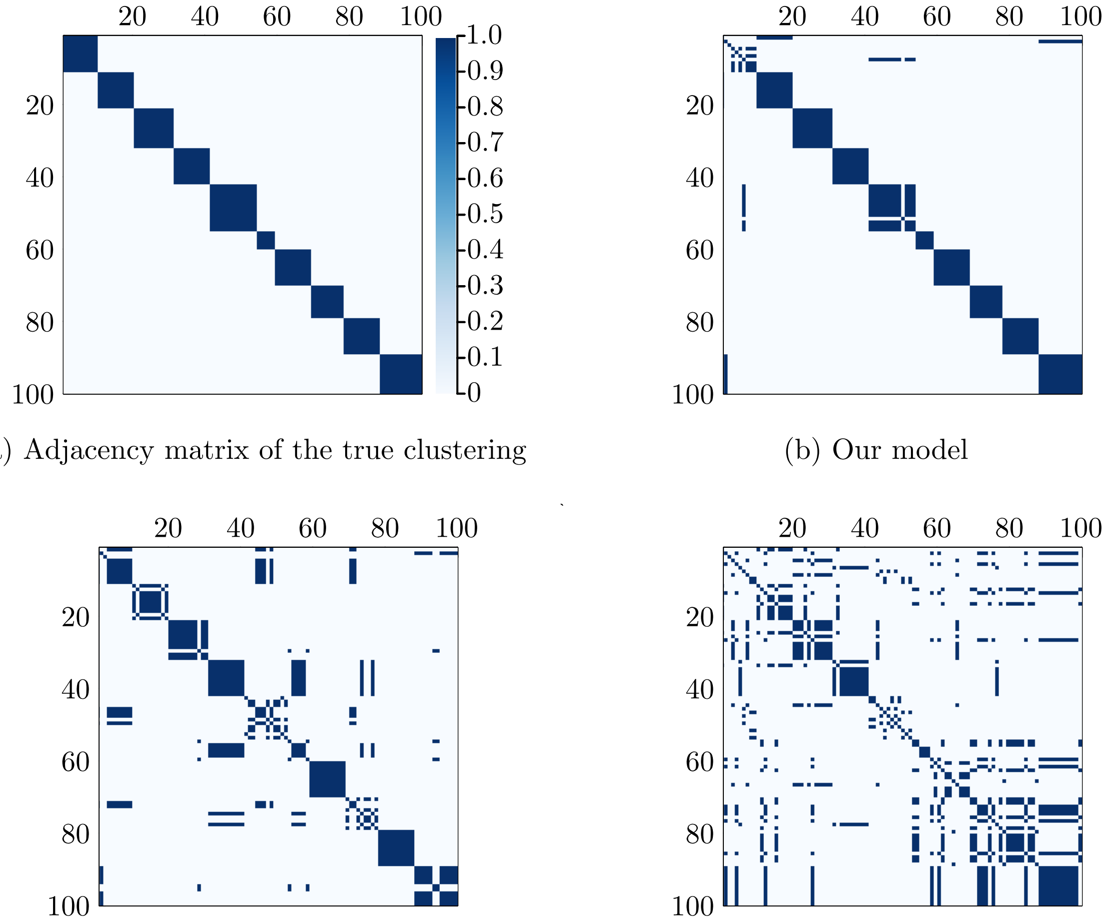


(a) Adjacency matrix of the true clustering

(b) Our model

(c) $k$-means

(d) $k$-medoids

Figure 17. Simulation study 2: Adjacency matrices of the point estimates. The point estimates obtained from the MFM and DPM results contained only a single cluster, so their adjacency matrices are not shown here.

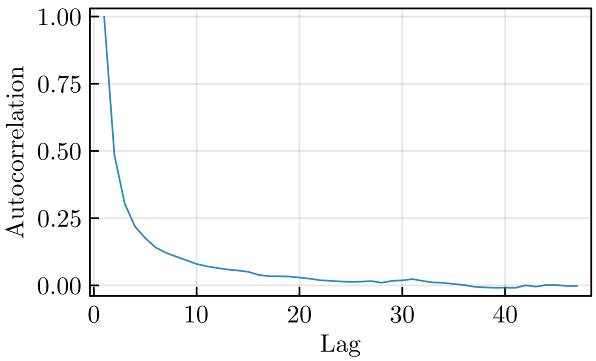


(a) $K$

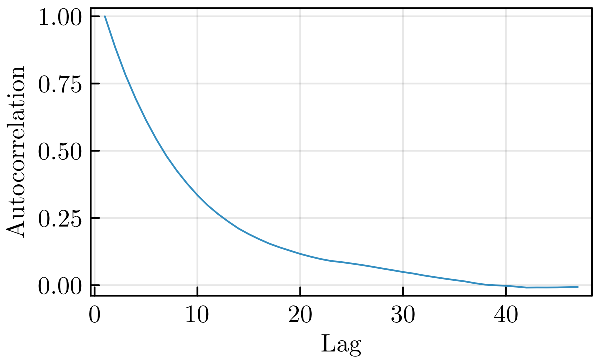


(b) $r$

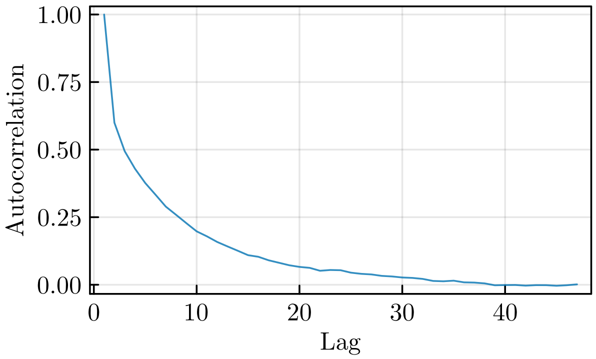


(c) $p$

Figure 18. Simulation study 2: Autocorrelation plots for $K$, $r$, and $p$

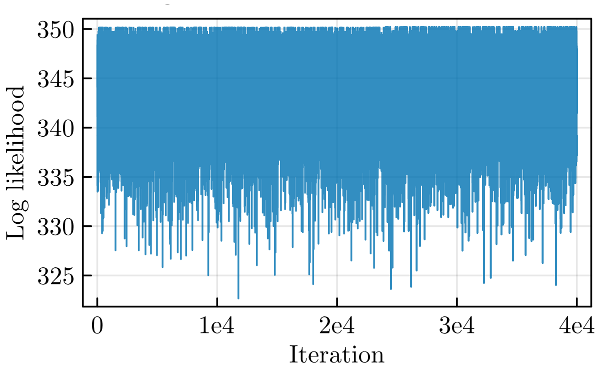


Figure 19. Simulation study 2: Log-likelihood trace-plot

| | Our Model | MFM | DPM | $k$-means | $k$-medoids |
|---|---|---|---|---|---|
| Binder loss | **0.02** | 0.9 | 0.9 | 0.06 | 0.13 |
| NVI distance | **0.06** | 0.5 | 0.5 | 0.18 | 0.42 |
| ARI | **0.90** | 0 | 0 | 0.66 | 0.34 |
| NMI | **0.94** | 0 | 0 | 0.82 | 0.57 |
| K | 13 | 1 | 1 | 13 | 13 |

Table 4. Simulation study 2: Clustering accuracy of point estimates with respect to the true clustering

| | IAC | ESS | ESR |
|---|---|---|---|
| K | 6.77 | 5907.80 | 0.15 |
| r | 17.88 | 2237.07 | 0.06 |
| p | 11.74 | 3408.48 | 0.09 |

Table 5. Simulation study 2: Convergence diagnostics

## 4.3 Simulation Study 3: Effect of Cluster Separation

In this example we show the effect of increased cluster separation by choosing $\sigma = 0.18$ and $d = 10$. Figure 20a shows that the pairwise Euclidean distances are better separated than in the previous two examples. Figure 21 shows the posterior distribution on the number of clusters for our model, our model without repulsion, MFM, and DPM. As expected, we underestimate uncertainty and get stuck in a local mode. This is because of the independence assumption on the distances within and between clusters, which causes an artificial peaking of the likelihood.

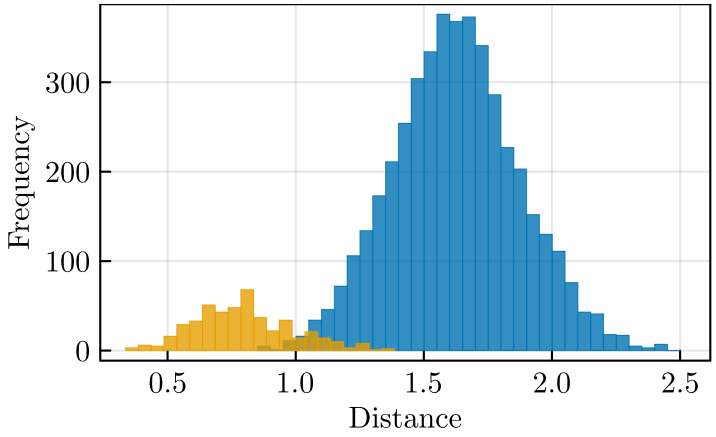


(a)

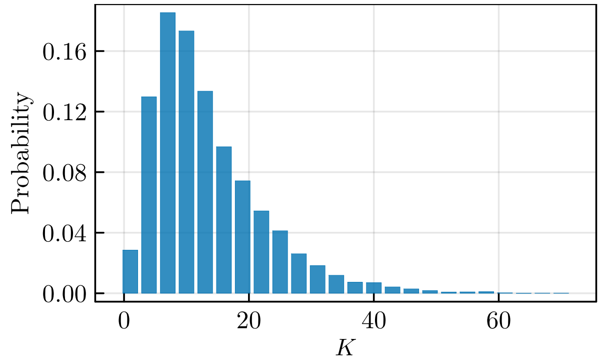


(b)

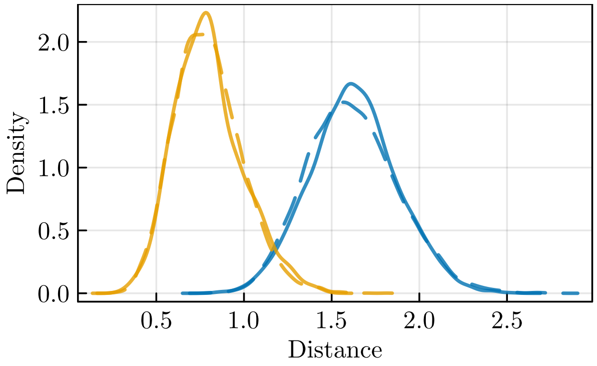


(c)

Figure 20. Simulated dataset 3: (a) Histogram of within-cluster distances (orange) and inter-cluster distances (blue). (b) Implied prior on the number of clusters $K$. (c) Predictive prior distribution (dashed lines) of the within-cluster distances (orange) and inter-cluster distances (blue) overlaid with the kernel density estimate of the true distances (solid lines).

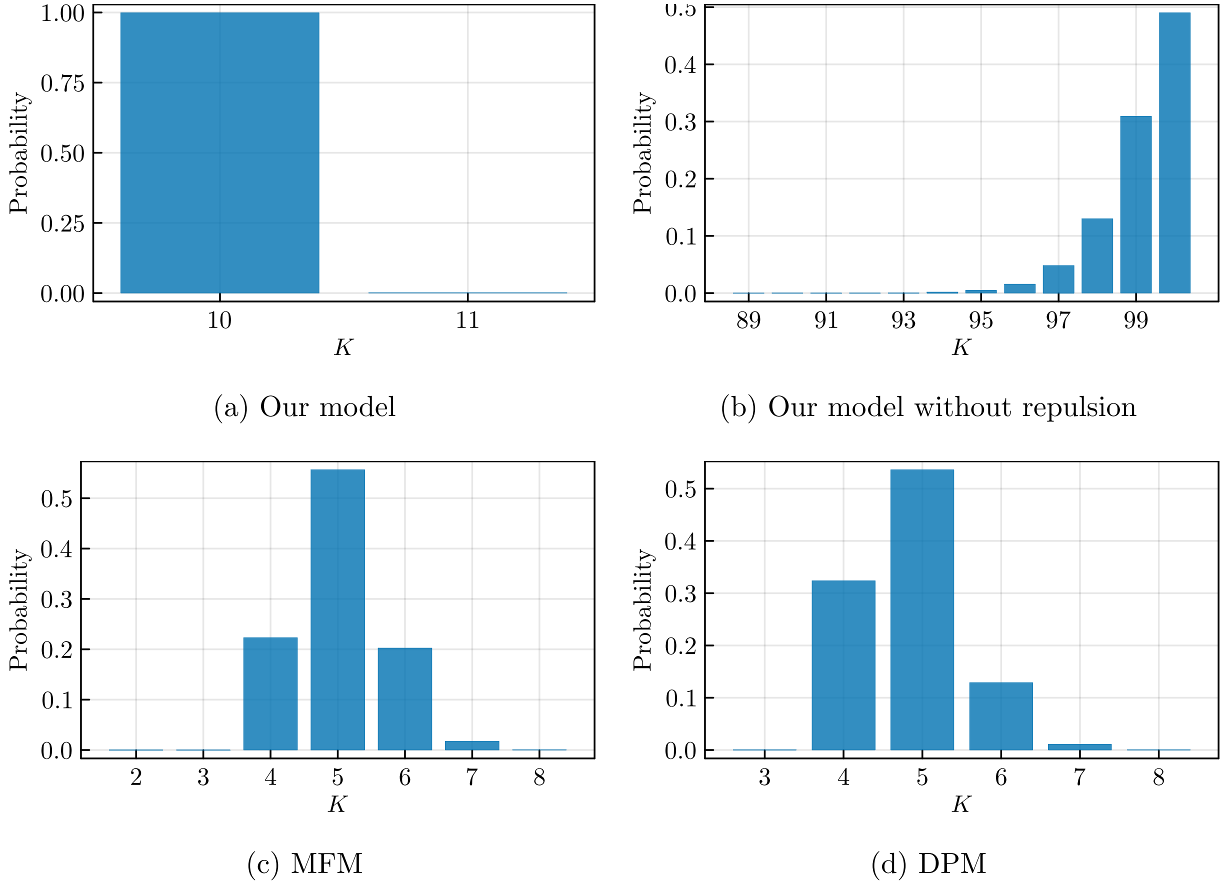


(a) Our model (b) Our model without repulsion

(c) MFM (d) DPM

Figure 21. Simulation study 3: Posterior distribution of the number of clusters $K$

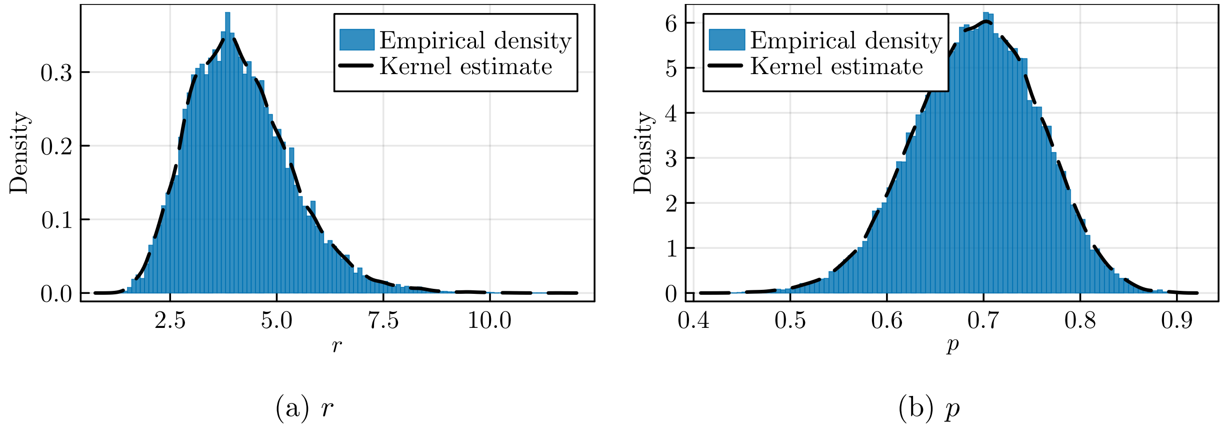


(a) $r$ (b) $p$

Figure 22. Simulation study 3: Posterior distribution of $r$ and $p$

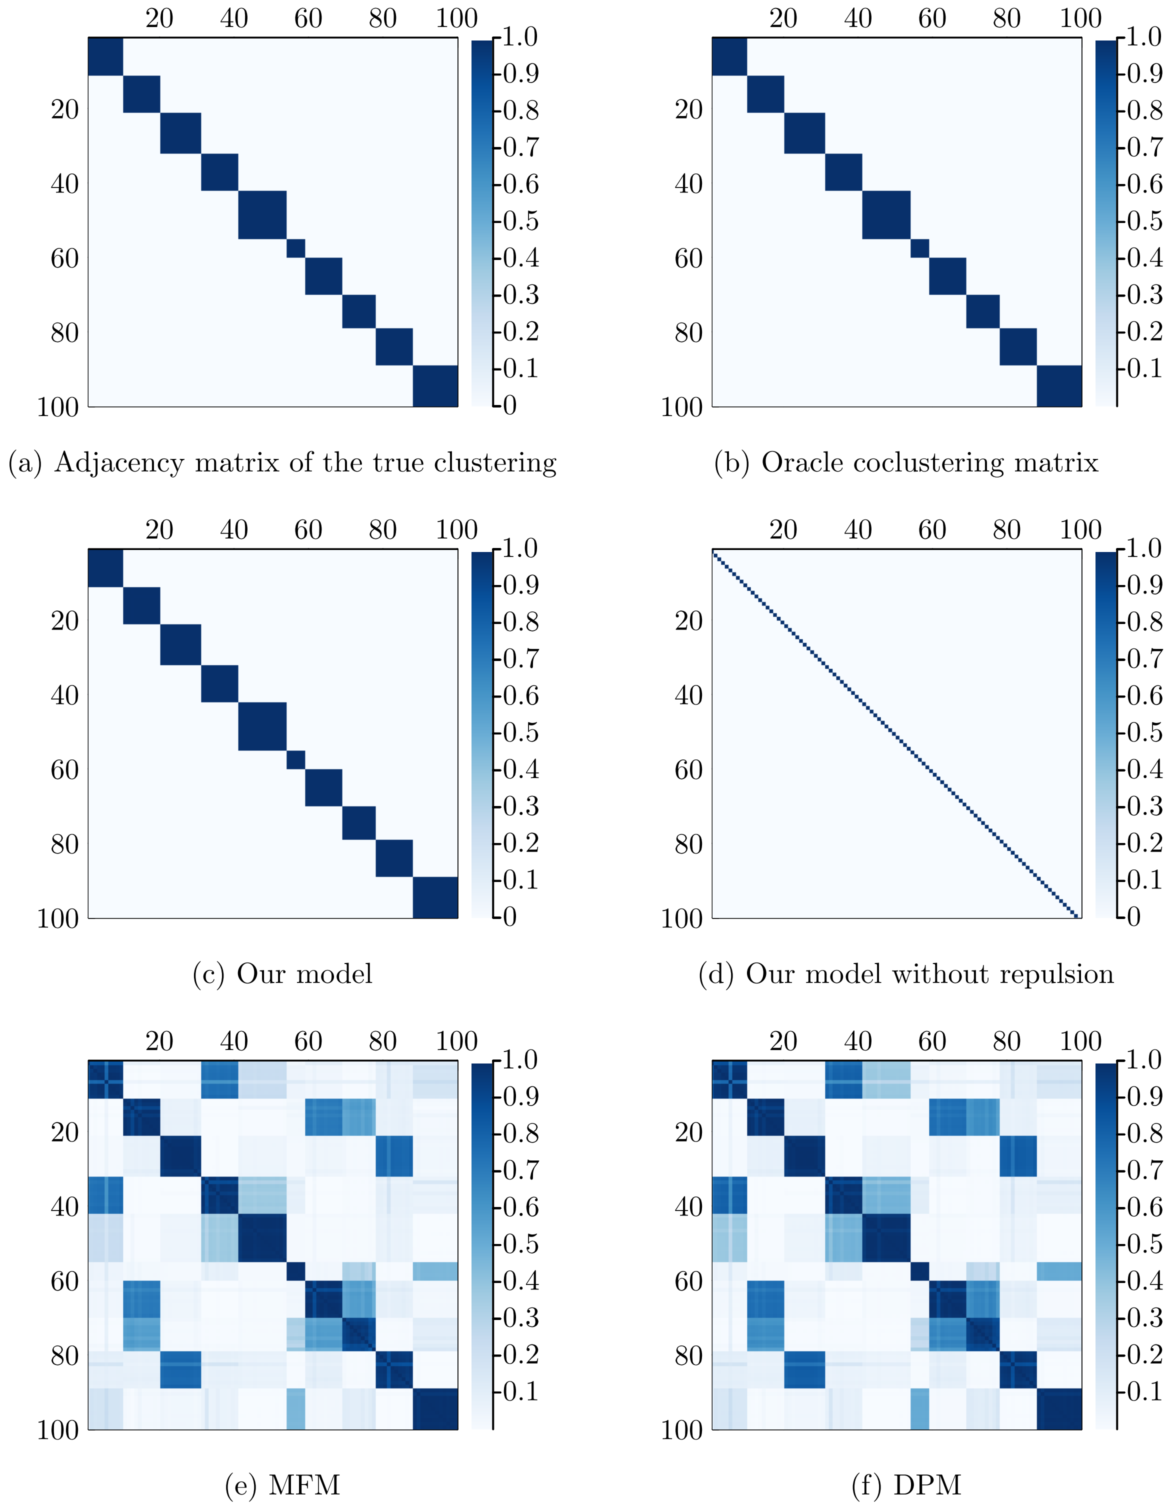

(a) Adjacency matrix of the true clustering

(b) Oracle coclustering matrix

(c) Our model

(d) Our model without repulsion

(e) MFM

(f) DPM

Figure 23. Simulation study 3: Posterior co-clustering matrices

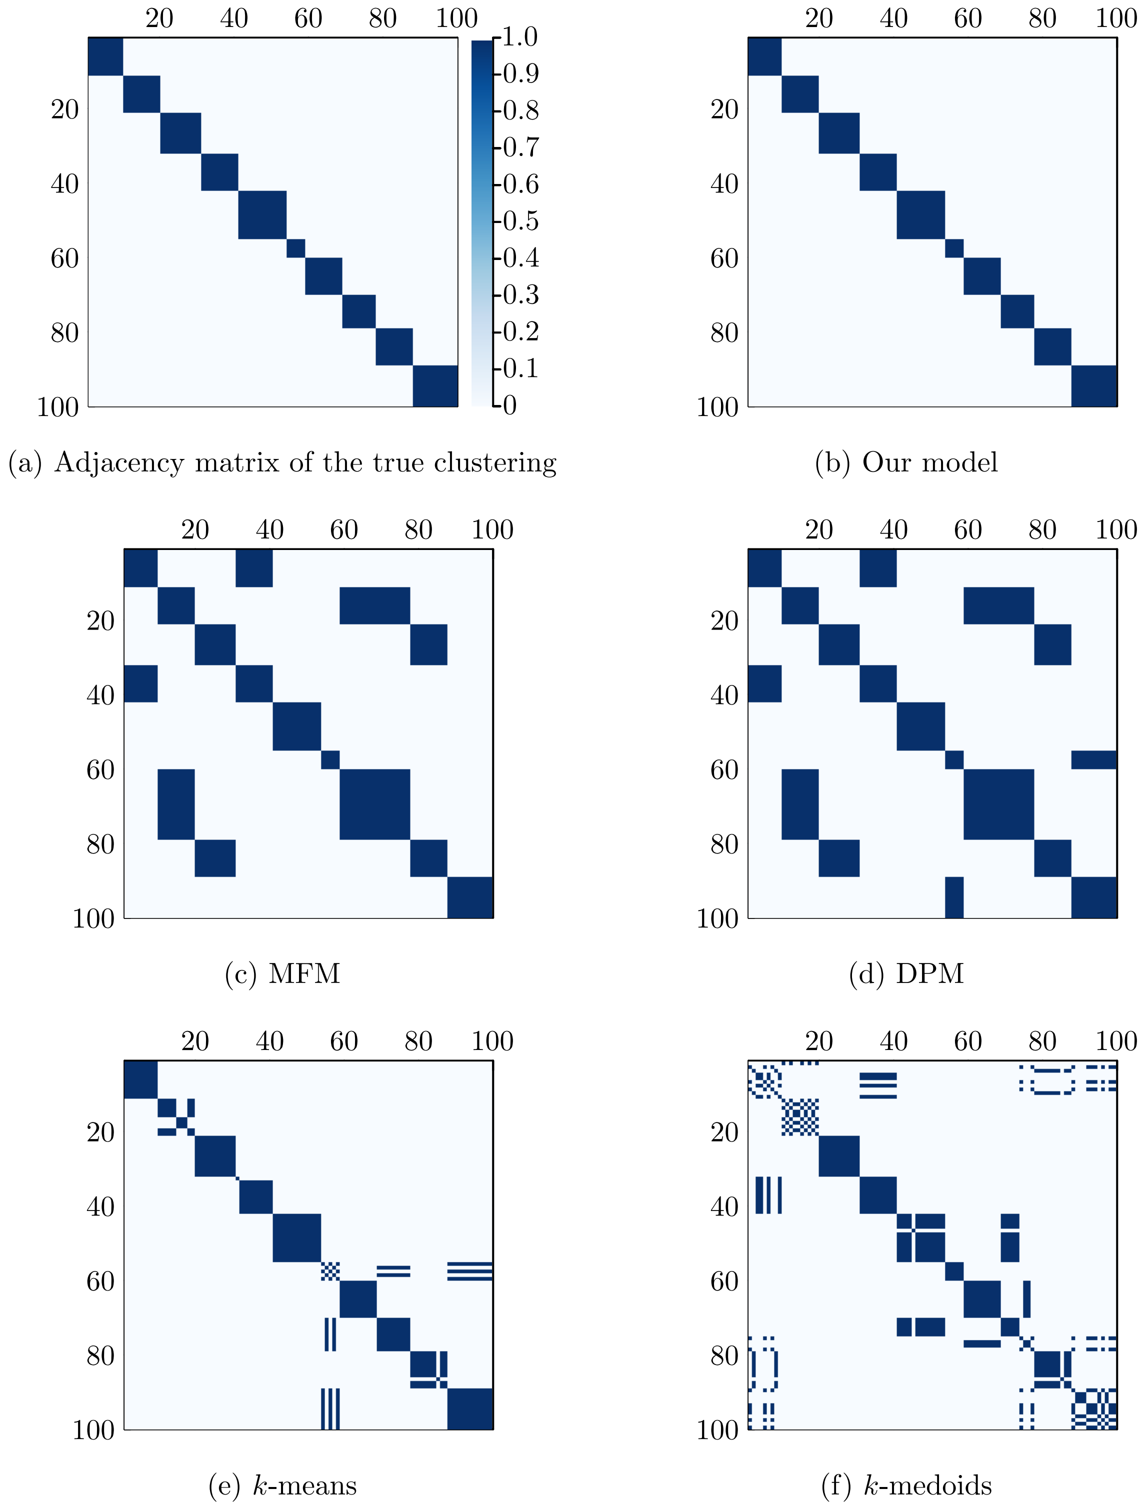


(a) Adjacency matrix of the true clustering

(b) Our model

(c) MFM

(d) DPM

(e) $k$-means

(f) $k$-medoids

Figure 24. Simulation study 3: Adjacency matrices of the point estimates

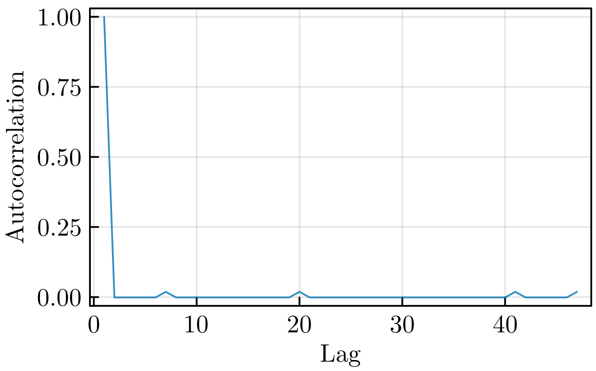


(a) $K$

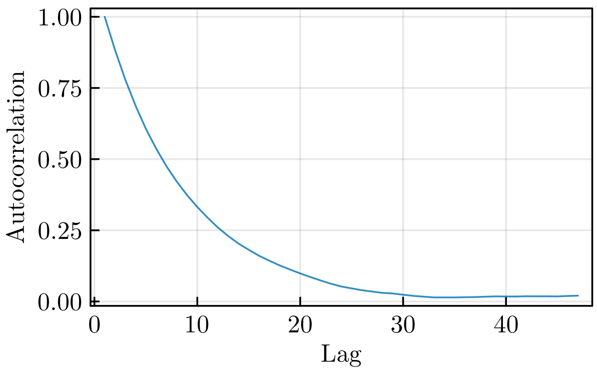


(b) $r$

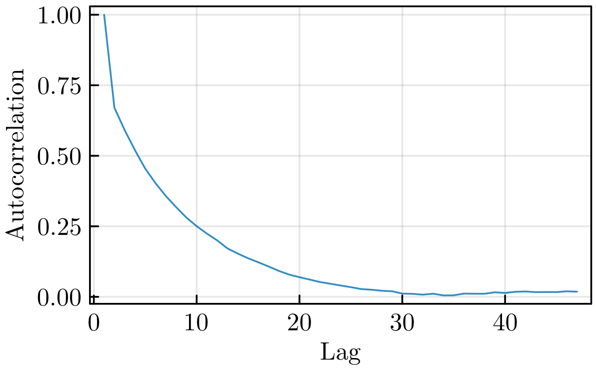


(c) $p$

Figure 25. Simulation study 3: Autocorrelation plots for $K$, $r$, and $p$

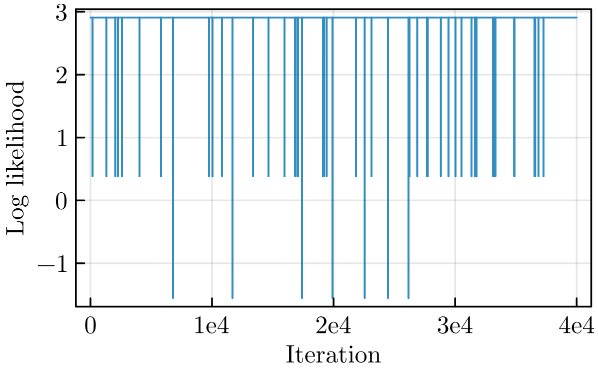


Figure 26. Simulation study 3: Log-likelihood trace-plot

| | Our Model | MFM | DPM | $k$-means | $k$-medoids |
|---|---|---|---|---|---|
| Binder loss | **0** | 0.1 | 0.11 | 0.02 | 0.07 |
| NVI distance | **0** | 0.13 | 0.15 | 0.06 | 0.19 |
| ARI | **1** | 0.6 | 0.58 | 0.88 | 0.63 |
| NMI | **1** | 0.85 | 0.82 | 0.94 | 0.81 |
| K | 10 | 6 | 5 | 12 | 12 |

Table 6. Simulation study 3: Clustering accuracy of point estimates with respect to the true clustering

| | IAC | ESS | ESR |
|---|---|---|---|
| K | 2.05 | 19560.01 | 0.49 |
| r | 17.35 | 2306.08 | 0.06 |
| p | 13.54 | 2954.95 | 0.07 |

Table 7. Simulation study 3: Convergence diagnostics

# 5 Choice of Prior Hyperparameters

## 5.1 Simulation Study 4: Robustness to Choice of Prior Hyperparameters

In this section we investigate posterior sensitivity to the choice of prior hyperparameters. The most important hyperparameters are those that determine the predictive distribution on the within-cluster and inter-cluster distances, which are in turn determined by the value of $K_{\text{elbow}}$ inferred by the elbow method. Given an objective function $\psi : [K_{\min}, K_{\max}] \to \mathbb{R}$, $K_{\text{elbow}}$ is given by

$$K_{\text{elbow}} = \underset{K \in [K_{\min}, K_{\max}]}{\arg\max} \|(K, \psi(K)) - \ell\|_2$$

where $\ell$ is the line joining $(K_{\min}, \psi(K_{\min}))$ and $(K_{\max}, \psi(K_{\max}))$ in $\mathbb{R}^2$.

The value of $K_{\text{elbow}}$ is affected by the algorithm used for the initial clustering ($k$-means, $k$-medoids), the objective function, and the range of values of $K$ over which the elbow method is applied. If the value of $K_{\text{elbow}}$ is too low, then the distribution on the within-cluster distances $f(x \mid \lambda_k)$ becomes over-dispersed while the distribution on inter-cluster distances becomes under-dispersed. The reverse happens if the value of $K_{\text{elbow}}$ is too large. This affects posterior inference on $K$ but the model still recovers the co-clustering structure well, as we show below. We run the model with the dataset from simulation study 1 (Section 4.1), but we artificially change the value picked by the elbow method ($K_{\text{elbow}} = 12$) to $K_{\text{elbow}} \pm 3$ before selecting the prior hyperparameters. Results are shown in Figures 27 to 31 and in Table 8.

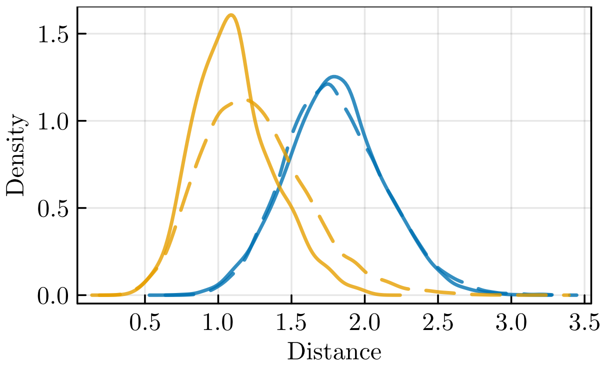


(a) $K_{\text{elbow}} = 9$

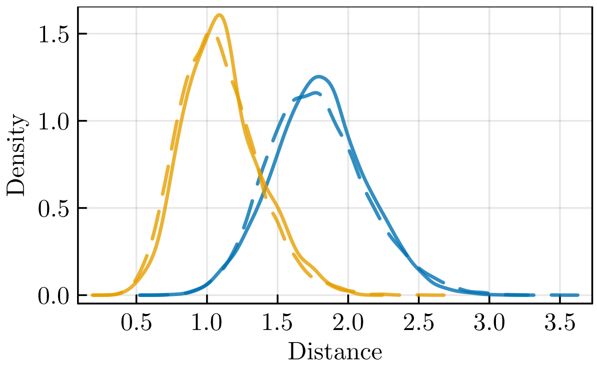


(b) $K_{\text{elbow}} = 15$

Figure 27. Simulation study 4: Predictive prior distribution (dashed lines) of the within-cluster distances (orange) and inter-cluster distances (blue) overlaid with the kernel density estimate of the true distances (solid lines).

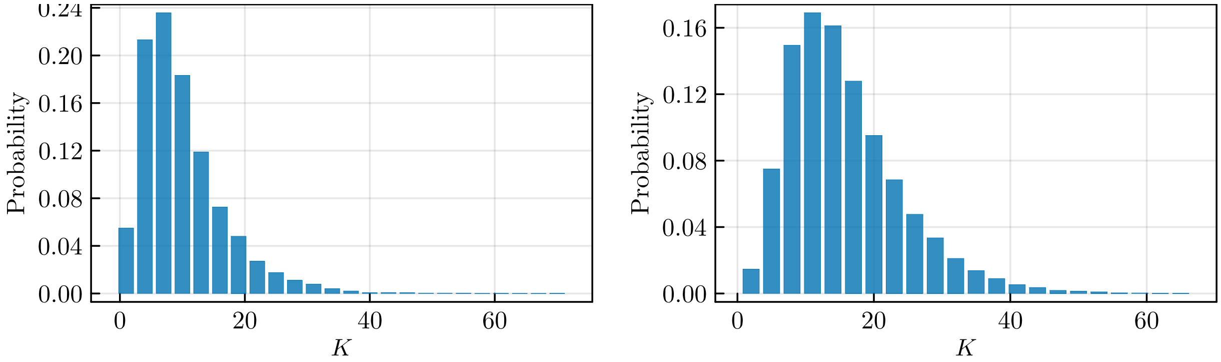


(a) $K_{\text{elbow}} = 9$ (b) $K_{\text{elbow}} = 15$

Figure 28. Simulation study 4: Implied prior predictive distribution on $K$

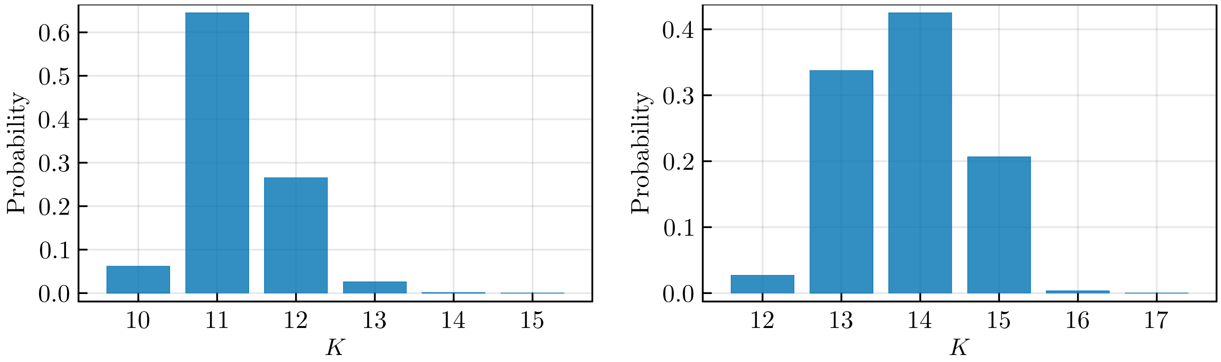


(a) $K_{\text{elbow}} = 9$ (b) $K_{\text{elbow}} = 15$

Figure 29. Simulation study 4: Posterior distribution on $K$

| $K_{\text{elbow}}$ : | 12 | 9 | 15 |
|---|---|---|---|
| Binder loss | 0.02 | 0.03 | **0.02** |
| NVI distance | 0.09 | 0.1 | **0.08** |
| ARI | 0.85 | 0.84 | **0.87** |
| NMI | 0.91 | 0.90 | **0.92** |
| K | 15 | 12 | 14 |

Table 8. Simulation study 4: Clustering accuracy of point estimates with respect to the true clustering

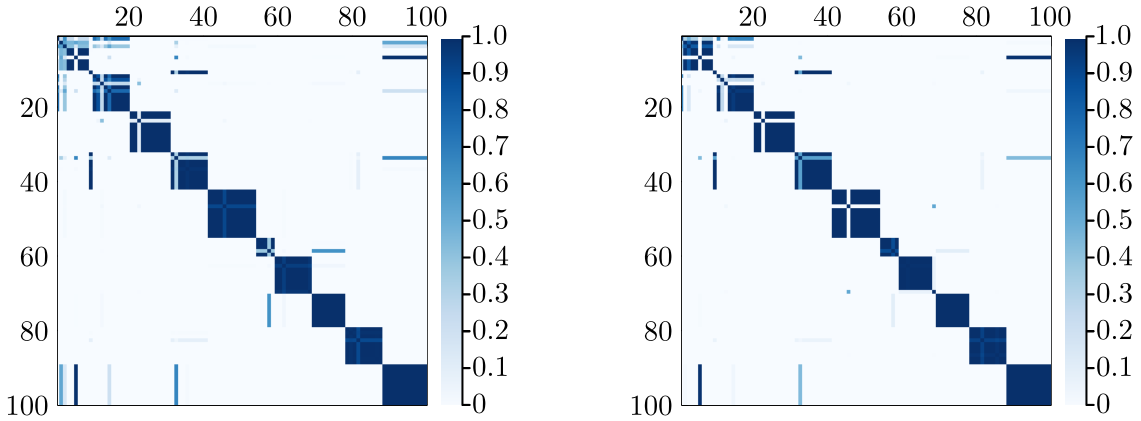


(a) $K_{\text{elbow}} = 9$ (b) $K_{\text{elbow}} = 15$

Figure 30. Simulation study 4: Posterior co-clustering matrices

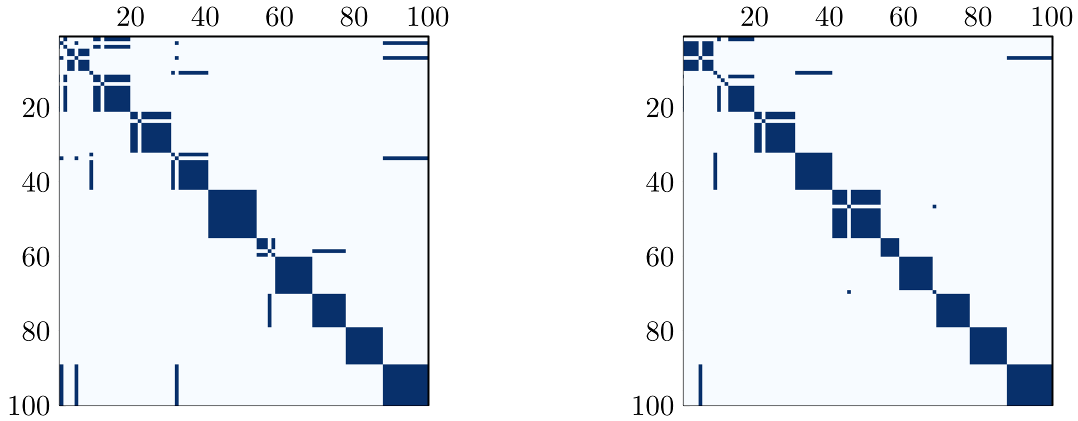


(a) $K_{\text{elbow}} = 9$ (b) $K_{\text{elbow}} = 15$

Figure 31. Simulation study 4: Adjacency matrices of the point estimates

## 5.2 Simulation Study 5: Alternative Method of Choosing Cluster-Specific Prior Hyperparameters

In this section we describe an alternative method to choose the prior hyperparameters for $\boldsymbol{\lambda}$ and $\boldsymbol{\theta}$ that reduces the dependence on the elbow method, and we test the method with a simulation study. The algorithm is a variation of Algorithm 1 from the main paper. The difference is that instead of partitioning the distances into within-cluster and inter-cluster distances for a fixed clustering configuration, we allow $K$ to vary and consider a mixture prior over all possible values of $K$.

**Algorithm 1** Alternative Method for Choosing $\alpha, \beta, \zeta, \gamma, \delta_1$, and $\delta_2$

1. Compute values for $\eta$, $\sigma$, $u$, and $v$ as in Algorithm 2 from the main paper.
2. Compute the implied prior predictive distribution on $K$ by generating samples from $\pi(K)$, using Equation (6) and a Gamma$(\eta, \sigma)$ prior on $r$ and Beta$(u, v)$ prior on $p$.
3. For each $K \in \{K_{\min}, \ldots, K_{\max}\}$, use $k$-means or $k$-medoids to obtain a clustering configuration $\rho^{(K)}$, and split the pairwise distances into two groups $A^{(K)}$ and $B^{(K)}$ that correspond to the within-cluster and inter-cluster distances in $\rho^{(K)}$. Here $K_{\min}$ and $K_{\max}$ correspond to the endpoints of the range of values over which the elbow method is applied in step 1.
4. Let $A$ and $B$ be the disjoint union of all the $A^{(K)}$ and $B^{(K)}$ respectively. Let $w_A$ and $w_B$ be importance weights associated to elements of $A$ and $B$, where $w_A(a) = \pi(K)$ if $a \in A^{(K)}$ and $w_B(b) = \pi(K)$ if $b \in B^{(K)}$.
5. Fit a Gamma distribution to the values in $A$ using weighted maximum likelihood estimation and set $\delta_1$ to be the shape parameter of this distribution.
6. Let $n_A = \sum_K \pi(K) n_{A^{(K)}}$, where $n_{A^{(K)}}$ is the cardinality of $A^{(K)}$. Set $\alpha = \delta_1 n_A$ and $\beta = \sum_{a \in A} w_A(a) a$, where $n_A$ is the cardinality of the set $A$.
7. Repeat steps 5 and 6 to obtain values for $\delta_2$, $\zeta$ and $\gamma$ by considering the values in $B$.

Step 6 of the algorithm corresponds to treating the elements $a_i \in A$ as observations from

the following model with an auxiliary weight variable $\boldsymbol{w}$:

$$\begin{aligned} w_i &\underset{\text{i.i.d}}{\sim} \text{Unif}(0,1) & 1 \le i \le \binom{|A|}{2} \\ \pi(\lambda) &\propto I(\lambda > 0) & \\ \pi(a_i \mid w_i, \lambda) &\propto f(a_i; \delta_1, \lambda)^{w_i} & 1 \le i \le \binom{|A|}{2} \end{aligned}$$

where $f(-;\delta_1,\lambda)$ is the density of the Gamma$(\delta_1,\lambda)$ distribution. In other words, we treat the data in $A$ that comes from $A^{(K)}$ as being observed with probability $\pi(K)$. Then the conditional posterior of $\lambda$ is given by

$$\pi(\lambda \mid A, \boldsymbol{w}) = \text{Gamma}\left(\delta_1 \sum_{a\in A} w_A(a), \sum_{a\in A} w_A(a)a\right)$$

### Simulation Results

In our simulation study we use the dataset from simulation study 1 (Section 4.1), set $K_{\min} = 1$, $K_{\max} = \lfloor n/2 \rfloor$, and we compare with those obtained with the original method. Results are shown in Figures 32 to 37 and in Table 9.

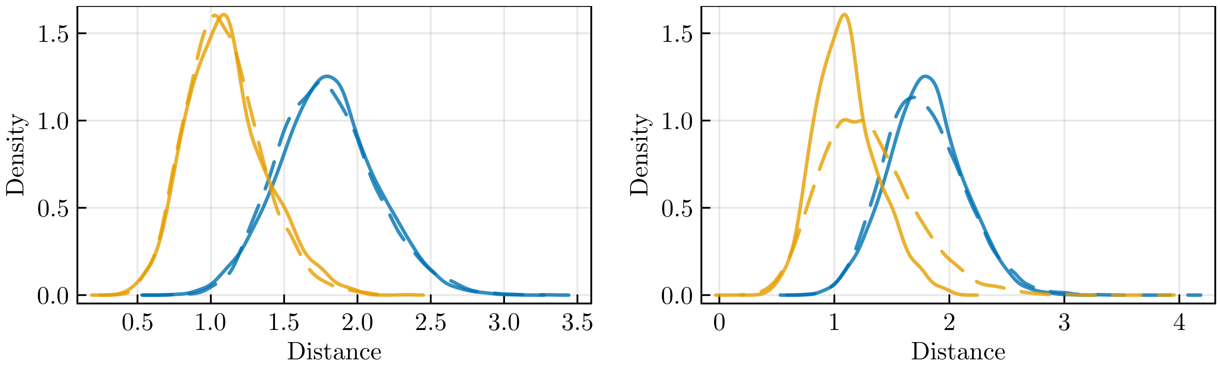


(a) Original method (b) Alternative method

Figure 32. Simulation Study 5: Predictive prior distribution (dashed lines) of the within-cluster distances (orange) and inter-cluster distances (blue) overlaid with the kernel density estimate of the true distances (solid lines).

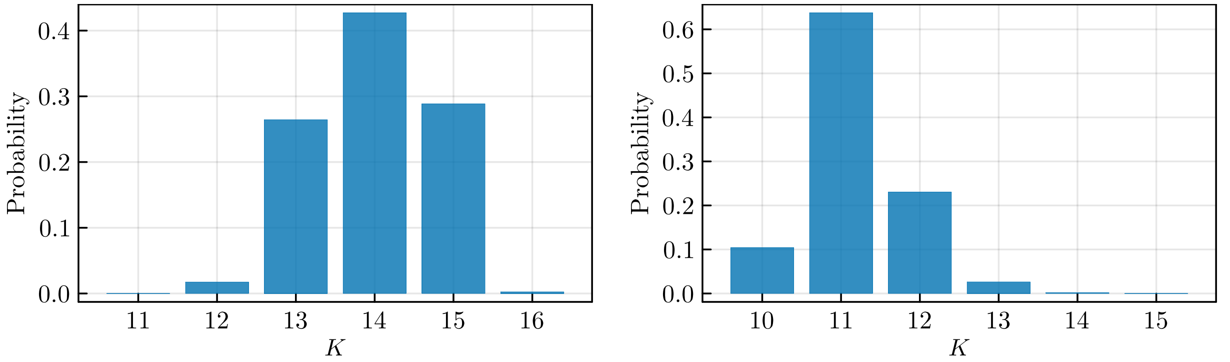


(a) Original method

(b) Alternative method

Figure 33. Simulation study 5: Posterior distribution of the number of clusters $K$

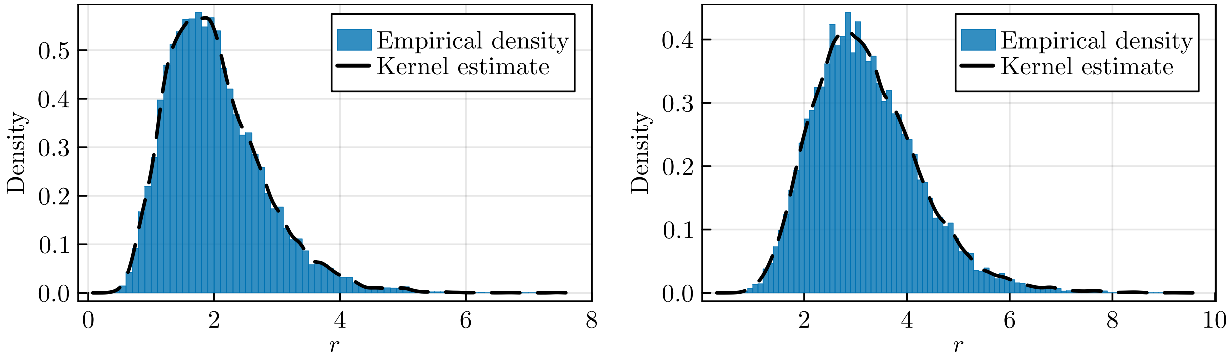


(a) Original method

(b) Alternative method

Figure 34. Simulation study 5: Posterior distribution of $r$

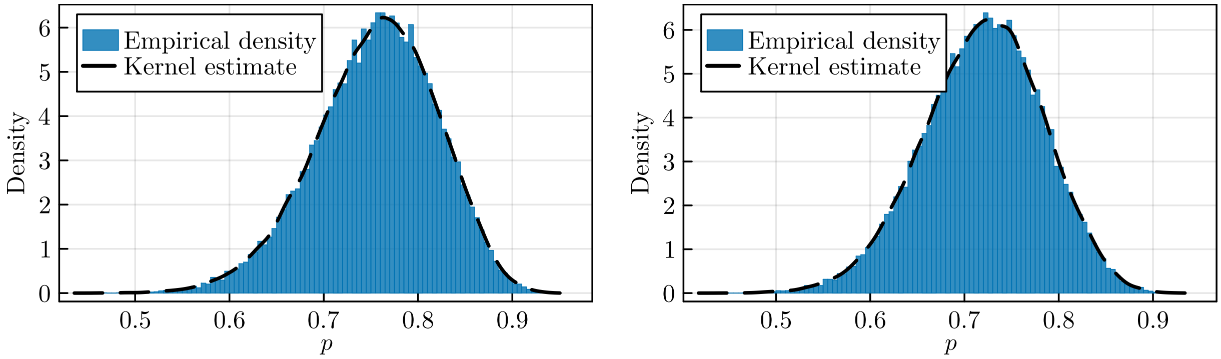


(a) Original method

(b) Alternative method

Figure 35. Simulation study 5: Posterior distribution of $p$

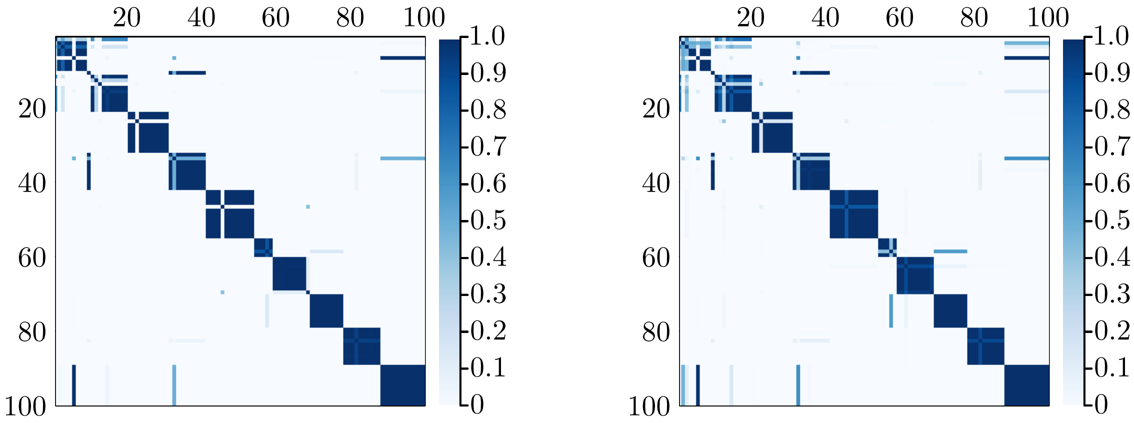


(a) Original method

(b) Alternative method

Figure 36. Simulation Study 5: Posterior co-clustering matrices

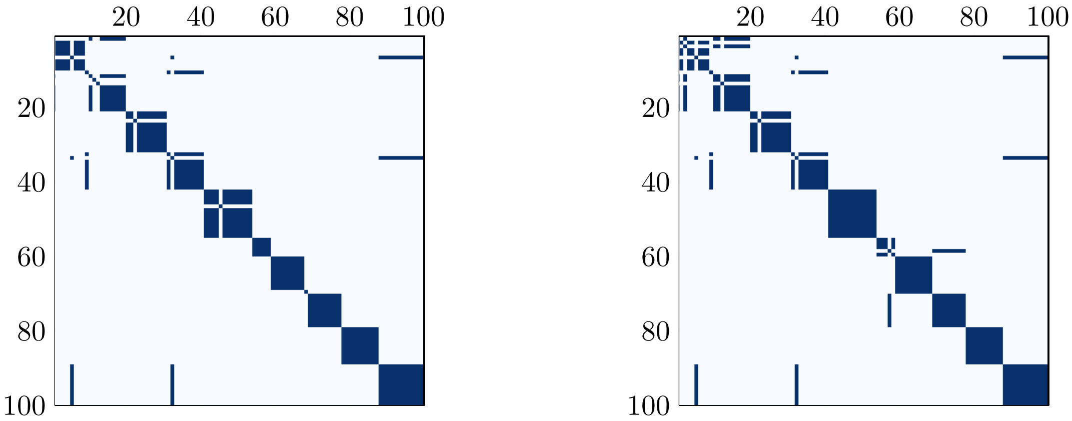


(a) Original method (b) Alternative method

Figure 37. Simulation Study 5: Adjacency matrices of the point estimates

| | Original method | Alternative method |
|---|---|---|
| Binder loss | 0.02 | **0.02** |
| VI distance | **0.09** | 0.09 |
| ARI | 0.85 | **0.86** |
| NMI | **0.91** | 0.91 |
| K | 15 | 12 |

Table 9. Simulation study 5: Clustering accuracy of point estimates with respect to the true clustering

# 6 Simulation Study 6: Role of Repulsion

In this section we show the importance of repulsion in our model. We run our model without repulsion on the data from simulation study 1 several times, varying the maximum number of clusters allowed. Figure 38 shows the posterior co-clustering matrix, and Figures 39 to 41 show the posterior distribution of $K$, $r$, and $p$ for each of these experiments. It is evident from Figure 39 that without repulsion, most of the posterior mass is concentrated near the maximum value allowed for $K$. This example as well previous simulated examples might lead to the belief that repulsion always leads to fewer clusters. However this is not the case, and depends on the scale of the data. For instance, if we rescale the distances in simulated example 1 to a maximum value less than one, the model instead coalesces all observations to a single cluster. We have noticed this behaviour on many simulations, including the coin example (results not shown). When there is no repulsion term, the marginal likelihood takes the form

$$\pi(\boldsymbol{D} \mid \rho_n) = \prod_{k=1}^{K} \frac{\Gamma(\alpha_k)}{\beta_k^{\alpha_k}} \prod_{\substack{i,j \in C_k \\ i<j}} \frac{D_{ij}^{\delta_1 - 1}}{\Gamma(\delta_1)}, \qquad \alpha_k = \alpha + n_k \delta_1, \qquad \beta_k = \beta + \sum_{i,j \in C_k} D_{ij}$$

When distances are concentrated in an interval $[0, a]$ with $a < 1$, the data-driven prior specification will (correctly) yield a prior predictive density for the within-cluster distances that is concentrated near zero, and this density will take values $> 1$ for the majority of distances in that interval. In this case the log marginal likelihood is maximised when all the distances are treated as being in the same cluster, whence the likelihood contribution from each distance will be greater than one. On the other hand if the distances are rescaled to an interval $[a, b]$ with $a > 1$, then the data-driven prior specification will yield a prior predictive density that takes values less than one for most of these distances. Consequently the log marginal likelihood is maximised when these distances are treated as being cross-cluster distances (i.e. every observation is its own cluster) whence there is no likelihood contribution from these distances (due to the lack of a repulsion term), and the log likelihood will be zero.

In other words the repulsion term acts as an identifiability constraint as well as making the model scale-invariant. We nevertheless recommend rescaling the distances to an interval $[a, b]$ with either $b < 1$ or $a > 1$.

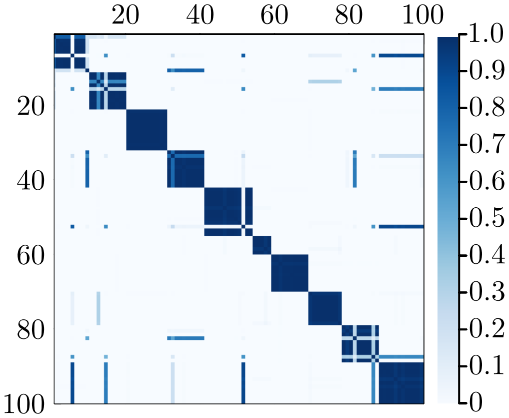


(a) max $K = 10$

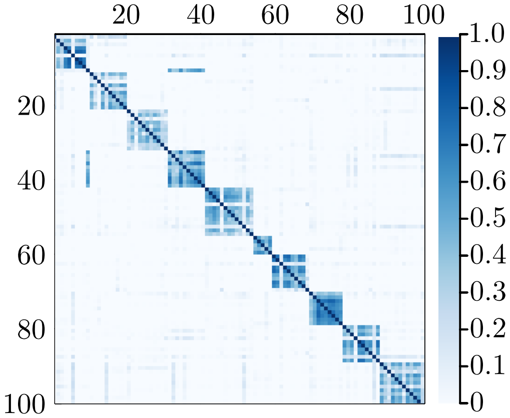


(b) max $K = 25$

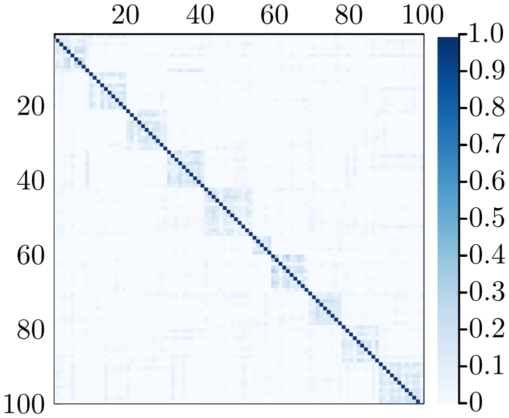


(c) max $K = 50$

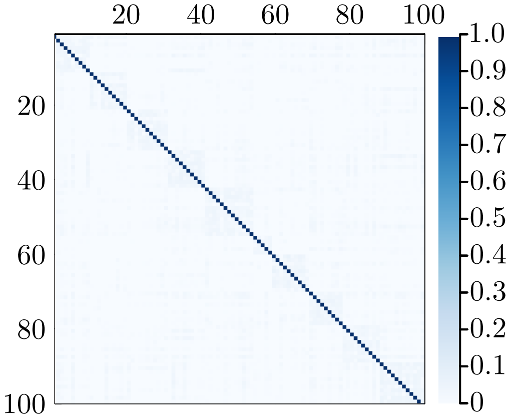


(d) max $K = 75$

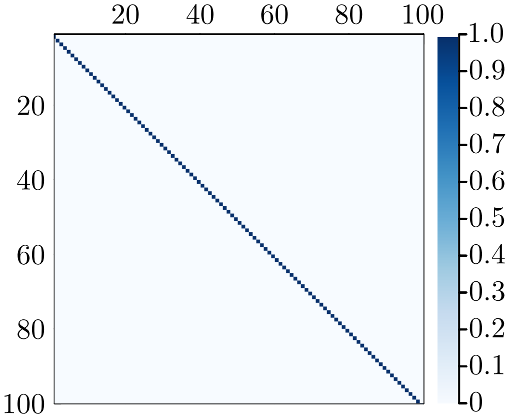


(e) max $K = 100$

Figure 38. Simulation study 6: Posterior co-clustering matrices

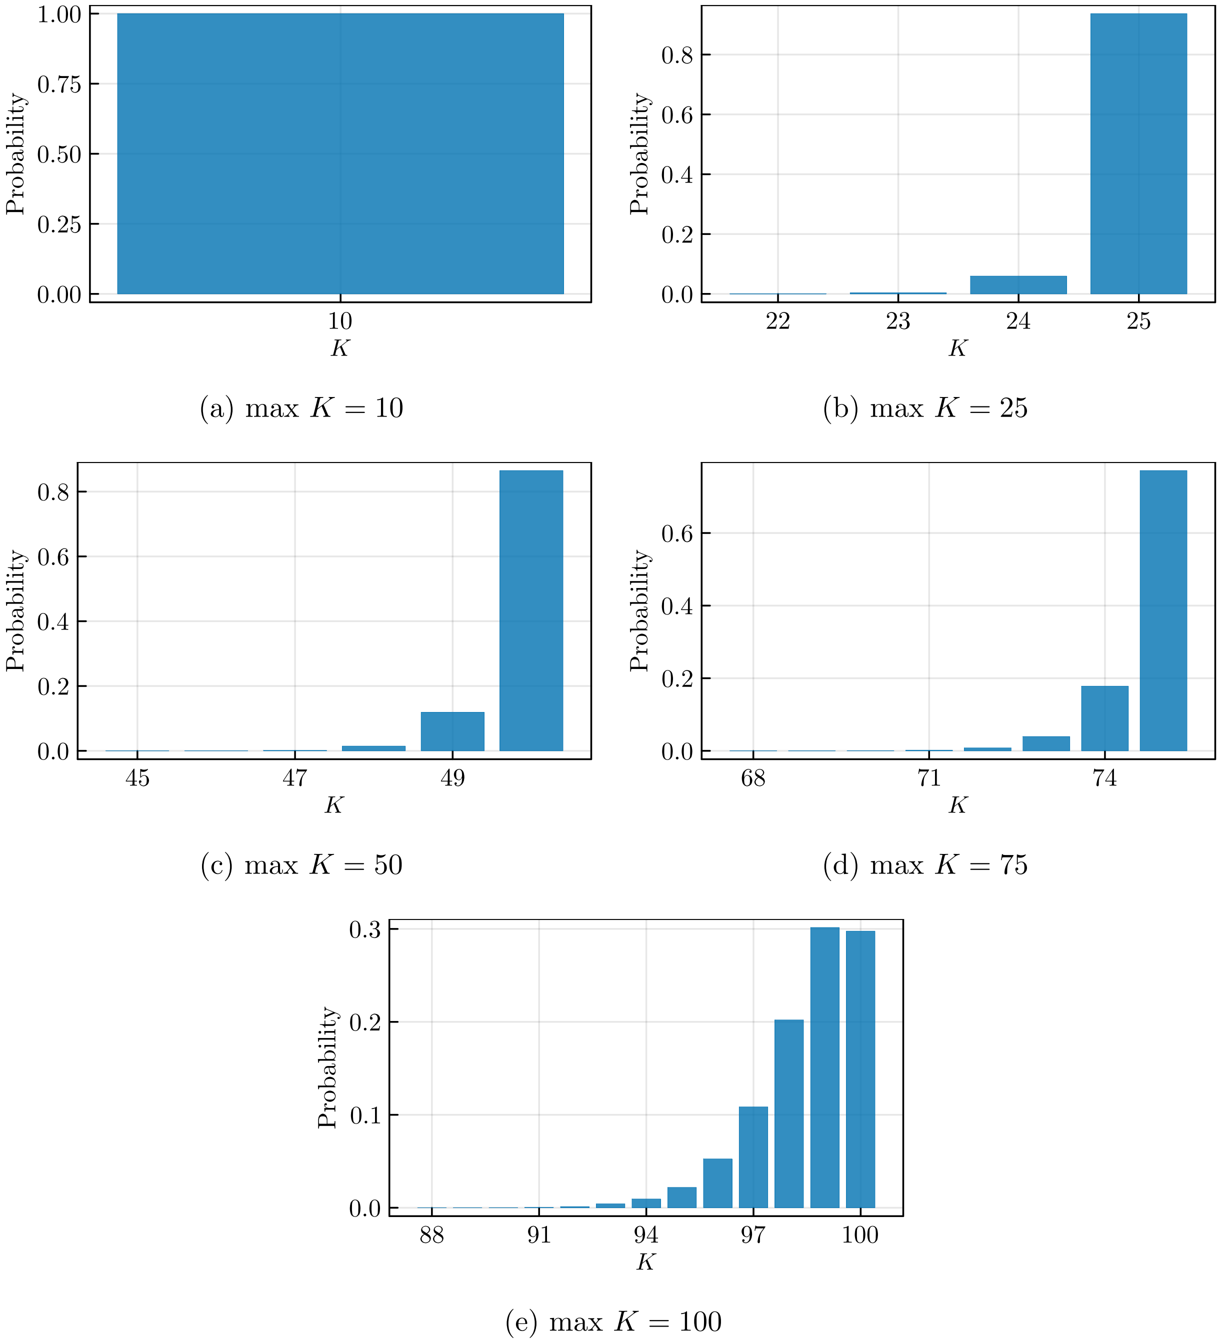


Figure 39. Simulation study 6: Posterior distribution on $K$

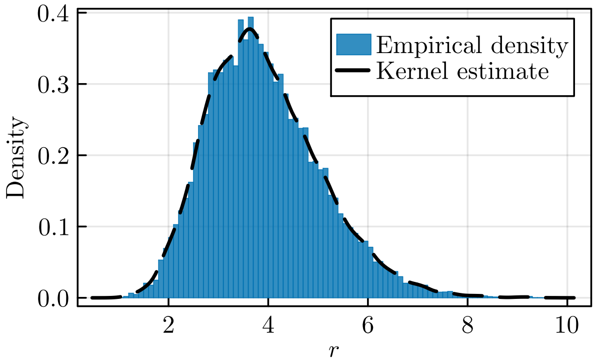


(a) max $K = 10$

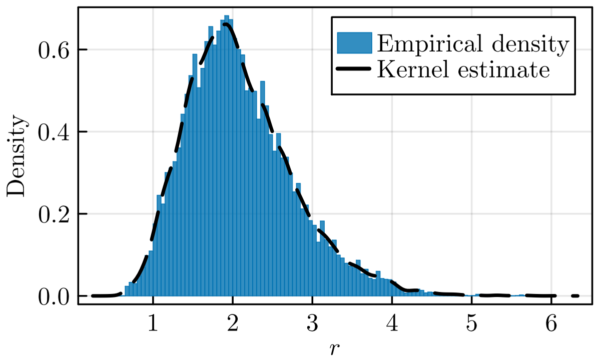


(b) max $K = 25$

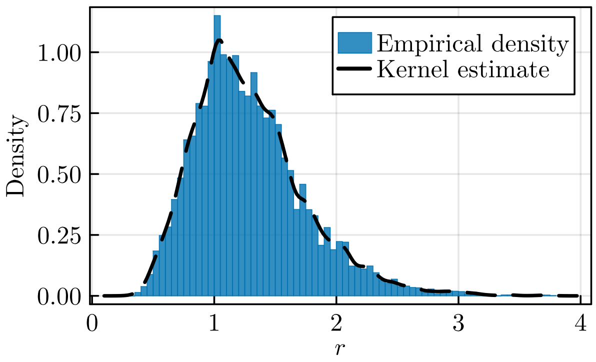


(c) max $K = 50$

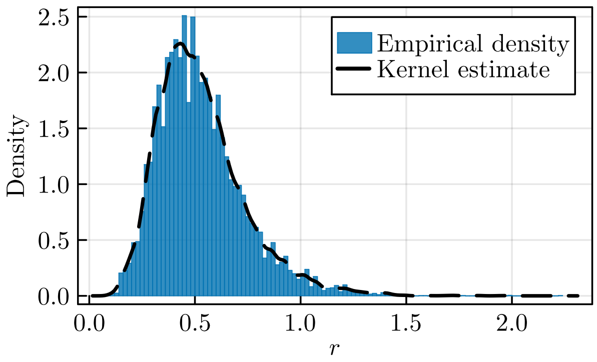


(d) max $K = 75$

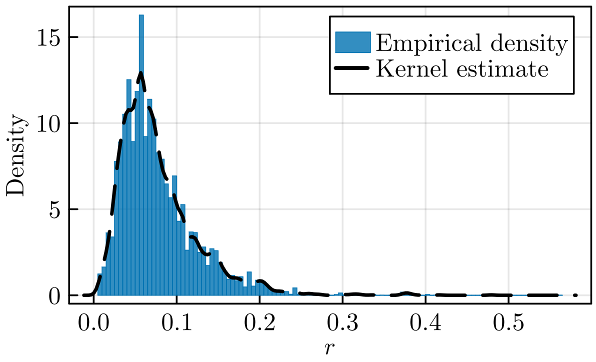


(e) max $K = 100$

Figure 40. Simulation study 6: Posterior distribution on $r$

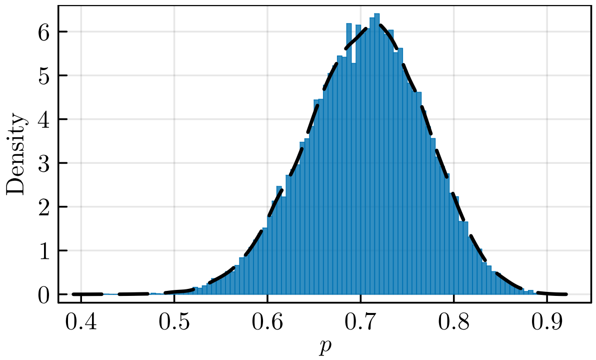


(a) max $K = 10$

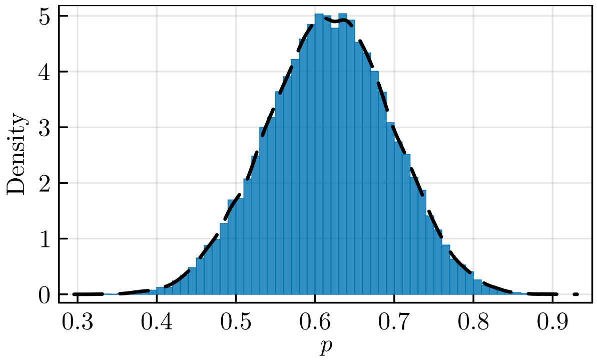


(b) max $K = 25$

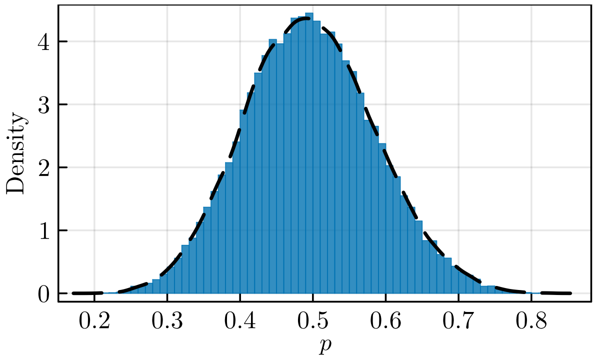


(c) max $K = 50$

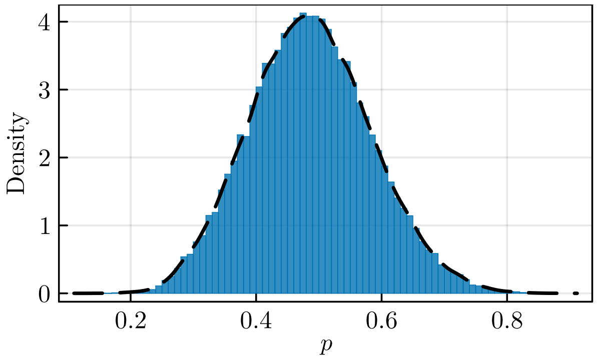


(d) max $K = 75$

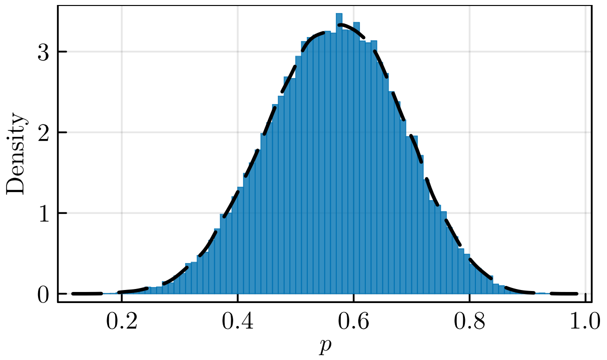


(e) max $K = 100$

Figure 41. Simulation study 6: Posterior distribution on $p$ and its kernel density estimate (dashed line)

# 7 Funding

This work was supported by the Singapore Ministry of Education through the Academic Research Fund Tier 2 under grant MOE-T2EP40121-0021, the National University of Singapore through the NUS HSS Seed Fund under grant R-607-000-449-646, by Yale-NUS College through Yale-NUS IG20-RA001.

# 8 Conflicts of Interest

We report that there are no competing interests to declare.

# References

Betancourt B, Zanella G, Steorts RC (2022). "Random Partition Models for Microclustering Tasks." *Journal of the American Statistical Association*, **117**(539), 1215–1227. doi:10.1080/01621459.2020.1841647.

Gao T, Kovalsky SZ, Daubechies I (2019). "Gaussian Process Landmarking on Manifolds." *SIAM Journal on Mathematics of Data Science*, **1**(1), 208–236. doi:10.1137/18M1184035.

Gower JC (1975). "Generalized procrustes analysis." *Psychometrika*, **40**(1), 33–51. doi:10.1007/BF02291478.

Gower JC, Dijksterhuis GB, *et al.* (2004). *Procrustes problems*, volume 30. Oxford University Press on Demand. ISBN 978-0198510581.

Gradshteyn I, Ryzhik I (2007). "Special Functions." In A Jeffrey, D Zwillinger (eds.), "Table of Integrals, Series, and Products (Seventh Edition)," chapter 8-9, pp. 859–1048. Academic Press, Boston, seventh edition. ISBN 978-0-12-373637-6. doi:10.1016/B978-0-08-047111-2.50016-9.

Jain S, Neal RM (2004). "A Split-Merge Markov chain Monte Carlo Procedure for the Dirichlet Process Mixture Model." *Journal of Computational and Graphical Statistics*, **13**(1), 158–182. doi:10.1198/1061860043001.

Lipman Y, Yagev S, Poranne R, Jacobs DW, Basri R (2014). "Feature Matching with Bounded Distortion." *ACM Transactions on Graphics*, **33**(3). ISSN 0730-0301. doi:10.1145/2602142.

Lowe D (2004). "Distinctive Image Features from Scale-Invariant Keypoints." *International Journal of Computer Vision*, **60**, 91–110. doi:10.1023/B:VISI.0000029664.99615.94.

Neal RM (2003). "Slice sampling." *The Annals of Statistics*, **31**(3), 705 – 767. doi:10.1214/aos/1056562461.

Pizer SM, Amburn EP, Austin JD, Cromartie R, Geselowitz A, Greer T, ter Haar Romeny B, Zimmerman JB, Zuiderveld K (1987). "Adaptive histogram equalization and its variations." *Computer vision, graphics, and image processing*, **39**(3), 355–368. doi:10.1016/S0734-189X(87)80186-X.

Rudin LI, Osher S, Fatemi E (1992). "Nonlinear total variation based noise removal algorithms." *Physica D: nonlinear phenomena*, **60**(1-4), 259–268. doi:10.1016/0167-2789(92)90242-F.
